# Supplementary material for: Deceptive, Disruptive, No Big Deal: Japanese People React to Simulated Dark Commercial Patterns
Source: arXiv:2405.08831 source file (2024-05-14)

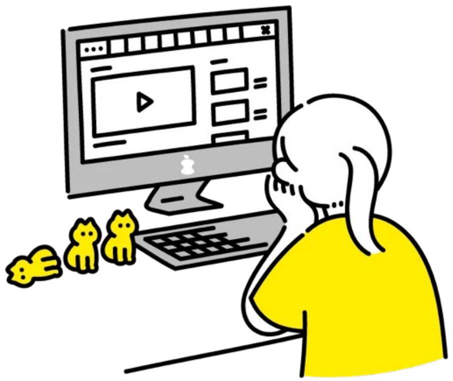

**Throughout**

途中

**Nagging**
Membership Nagging

**Interface Interference**
Hidden Information
False Hierarchy
Toying with Emotions

**Linguistic Dead-Ends**
Untranslation
Alphabet Soup

## 1

**Browse the homepage**

ホームページを見る

**Interface Interference**
Hidden Information
False Hierarchy
Toying with Emotions

**Social Proof**
Notification of Others’ Activities

**Urgency**
Countdown Timer

**Nagging**
Membership Nagging ×2

## 2

**Browse the shop for a set of items**

ショップでセットを作る

**Interface Interference**
Preselection
False Hierarchy
Hidden Information
Disguised Advertisements
Toying with Emotions
Misleading Reference Pricing

**Sneaking**
Sneaking an Item

**Social Proof**
Testimonials
Notification of Others’ Activities

**Nagging**
Turn On Location-Tracking

## 3

**Check-out and sign up**

チェックアウトとサインアップ

**Forced Action**
Forced to Register

**Sneaking**
Drip Pricing
Hidden Subscription

**Interface Interference**
Preselection
Hidden Information
False Hierarchy
Trick Questions

**Urgency**
Low Stock/High Demand
Countdown Timer

**Linguistic Dead-Ends**
Alphabet Soup

## 4

**Cancel your membership**

会員およびアカウントの解約

**Obstruction**
Hard to Cancel

**Interface Interference**
Confirmshaming
Toying with Emotions
False Hierarchy

**Linguistic Dead-Ends**
Untranslation

途中

Throughout

途中

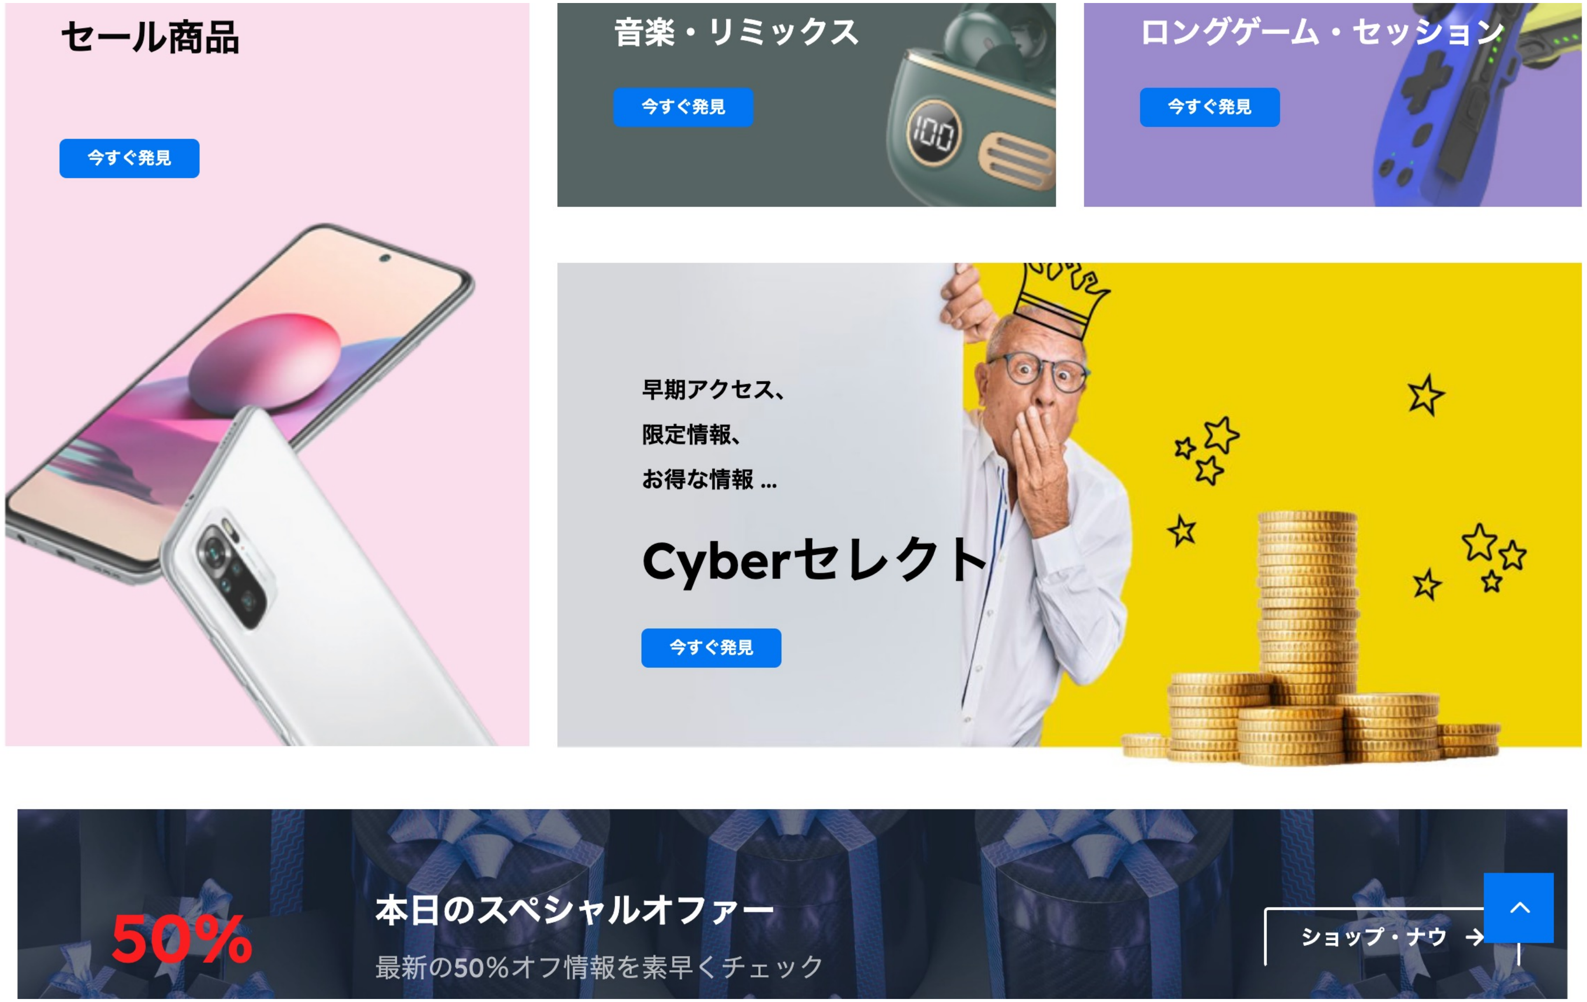

途中

Throughout

途中

**Nagging**

Membership Nagging

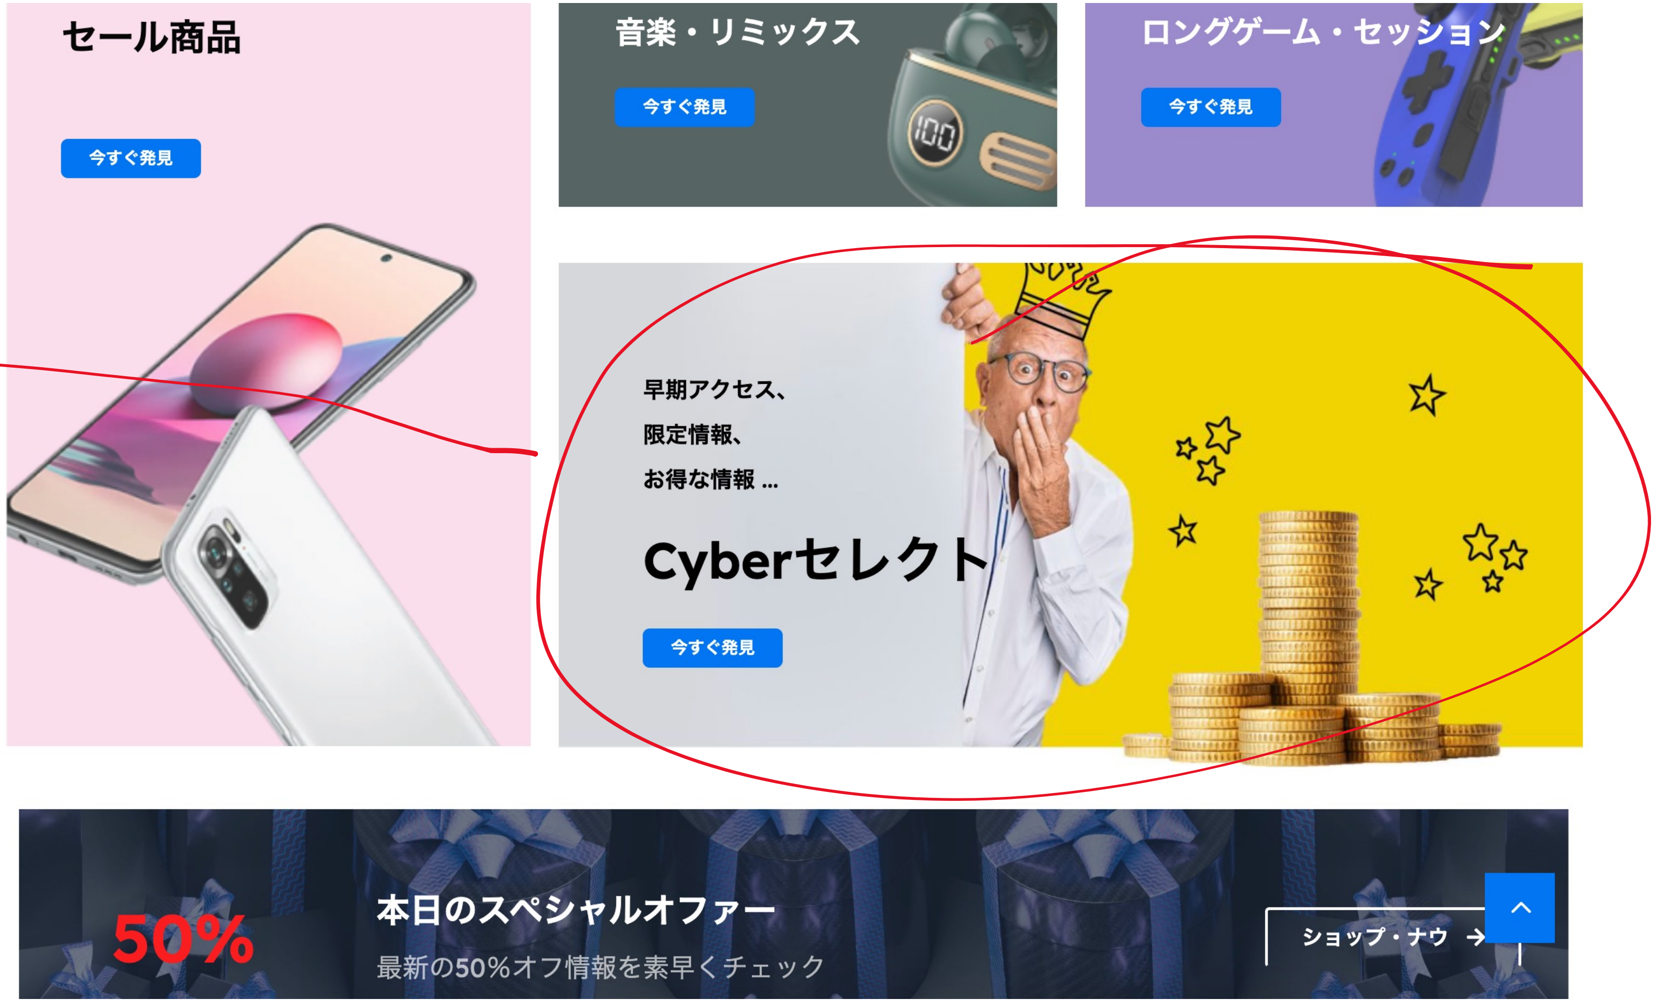

途中

Throughout

途中

## ミニマムプラン

**¥99.5** /年

**標準的なプラン**

- ✔ **限定** 送料無料
- ✔ OLUゴールへのアクセス**制限**
- ✔ **限定** お買い得情報

## ベーシックプラン

**¥129.5** /年

**一番人気、一番お買い得**

- ✔ **無制限** 送料無料
- ✔ **無制限** OLUゴールへのアクセス
- ✔ **無制限** お買い得情報
- ✔ 会員特別価格

## ノープラン

**¥0** /年

**普通**

- ✘ 送料無料**なし**
- ✘ OLUゴールへのアクセス**なし**
- ✔ **限定** お買い得情報

**登録はこちらから**

途中

Throughout

途中

**Nagging**

Membership Nagging

**Interface Interference**

Hidden Information

False Hierarchy

Toying with Emotions

**Linguistic Dead-Ends**

Alphabet Soup

## ミニマムプラン

¥99.5 /年

標準的なプラン

✔ 限定 送料無料

✔ OLUゴールへのアクセス制限

✔ 限定 お買い得情報

## ベーシックプラン

¥129.5 /年

一番人気、一番お買い得

✔ 無制限 送料無料

✔ 無制限 OLUゴールへのアクセス

✔ 無制限 お買い得情報

✔ 会員特別価格

## ノープラン

¥0 /年

普通

✘ 送料無料なし

✘ OLUゴールへのアクセスなし

✔ 限定 お買い得情報

登録はこちらから

途中

Throughout

途中

CyberStore

すべてのカテゴリー

検索 ...

¥0 - 0点

🎁 商品　👑 Cyberセレクト

マイアカウント

# 利用条件

ホーム / 利用条件

**利用規約とプライバシーポリシーをよくお読みください。**

## Overview

Our refund and returns policy lasts 30 days. If 30 days have passed since your purchase, we can’t offer you a full refund or exchange.

To be eligible for a return, your item must be unused and in the same condition that you received it. It must also be in the original packaging.

Several types of goods are exempt from being returned. Perishable goods such as food, flowers, newspapers or magazines cannot be returned. We also do not accept products that are intimate or sanitary goods, hazardous materials, or flammable liquids or gases.

Additional non-returnable items:

途中

Throughout

途中

**Linguistic Dead-Ends**

Untranslation

CyberStore

すべてのカテゴリー

検索 ...

¥0 - 0点

商品 Cyberセレクト マイアカウント

# 利用条件

ホーム / 利用条件

**利用規約とプライバシーポリシーをよくお読みください。**

## Overview

Our refund and returns policy lasts 30 days. If 30 days have passed since your purchase, we can't offer you a full refund or exchange.

To be eligible for a return, your item must be unused and in the same condition that you received it. It must also be in the original packaging.

Several types of goods are exempt from being returned. Perishable goods such as food, flowers, newspapers or magazines cannot be returned. We also do not accept products that are intimate or sanitary goods, hazardous materials, or flammable liquids or gases.

Additional non-returnable items:

1

Browse the homepage

ホームページを見る

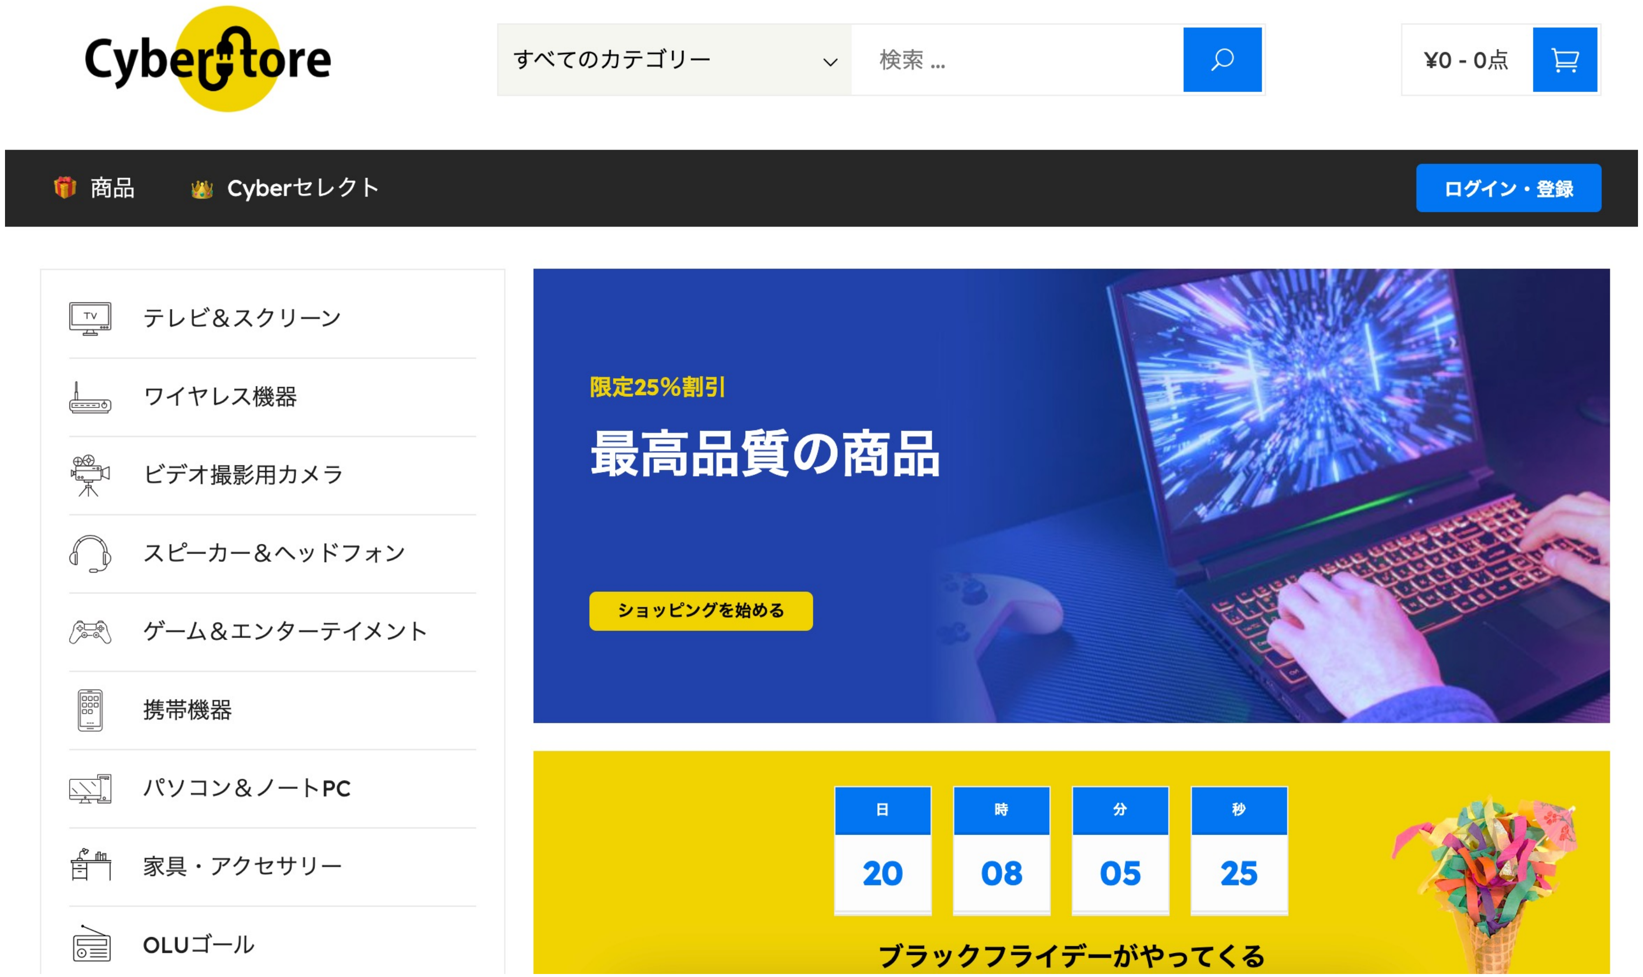

1

Browse the homepage

ホームページを見る

**Interface Interference**

Hidden Information

False Hierarchy

Toying with Emotions

**Social Proof**

Notification of Others’ Activities

**Urgency**

Countdown Timer

**Nagging**

Membership Nagging

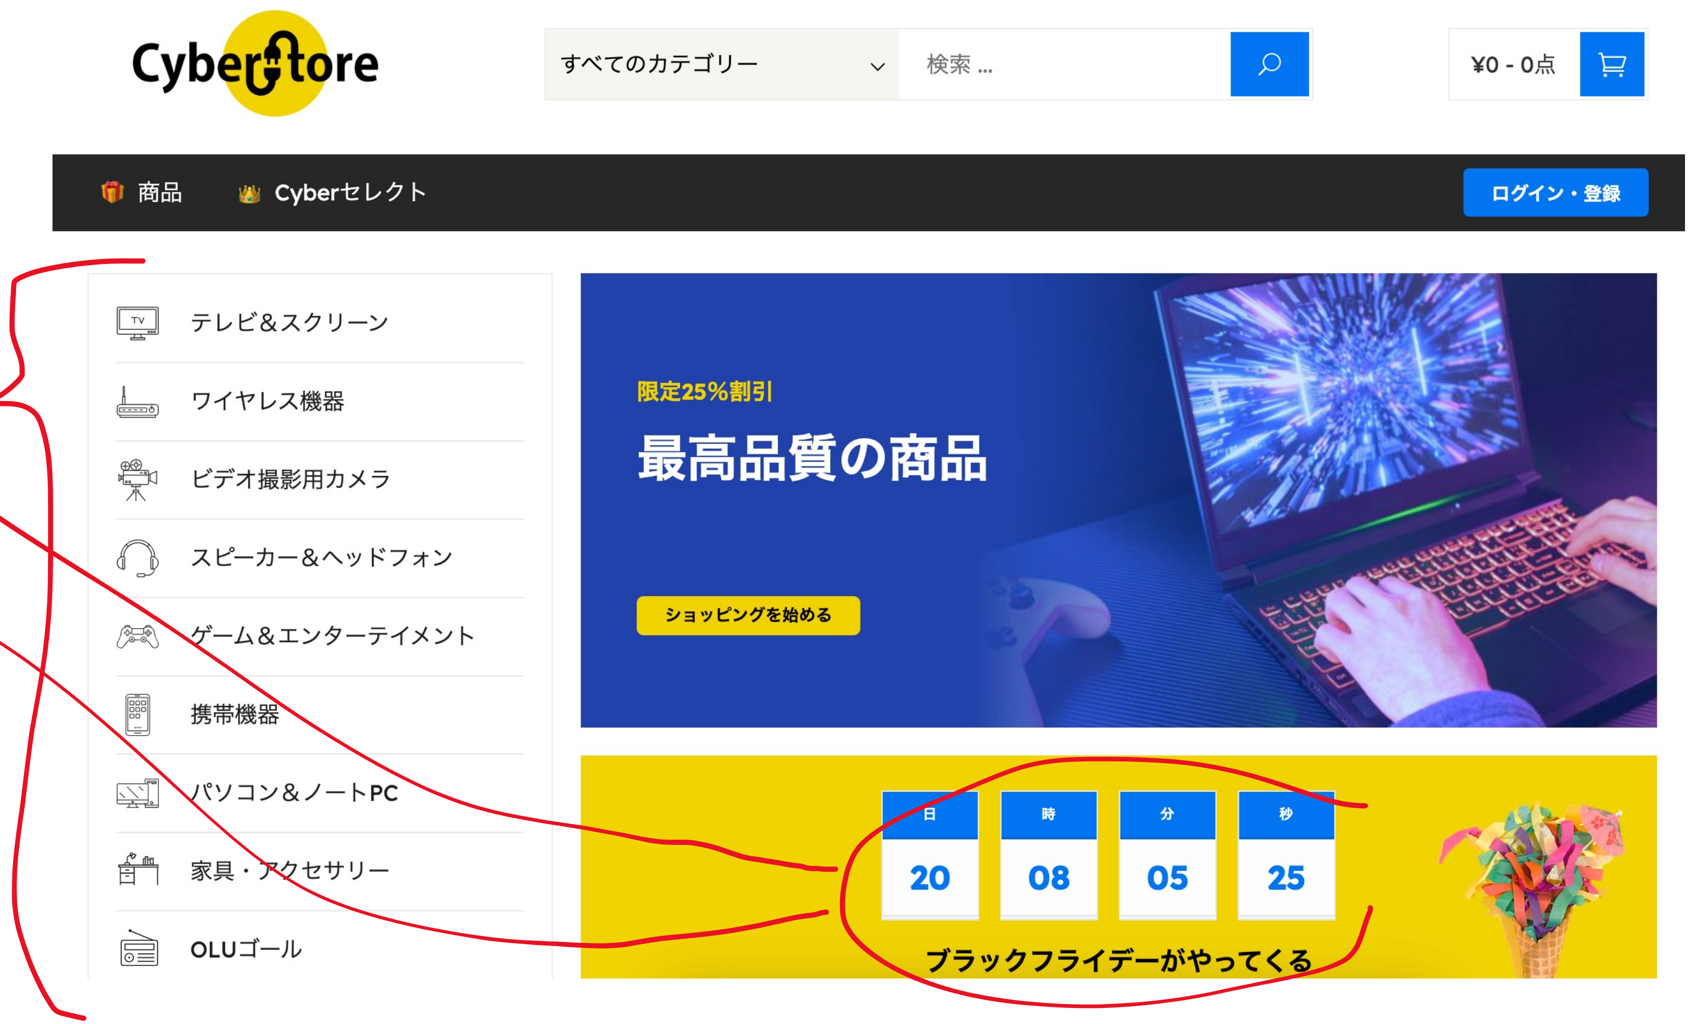

1

Browse the homepage

ホームページを見る

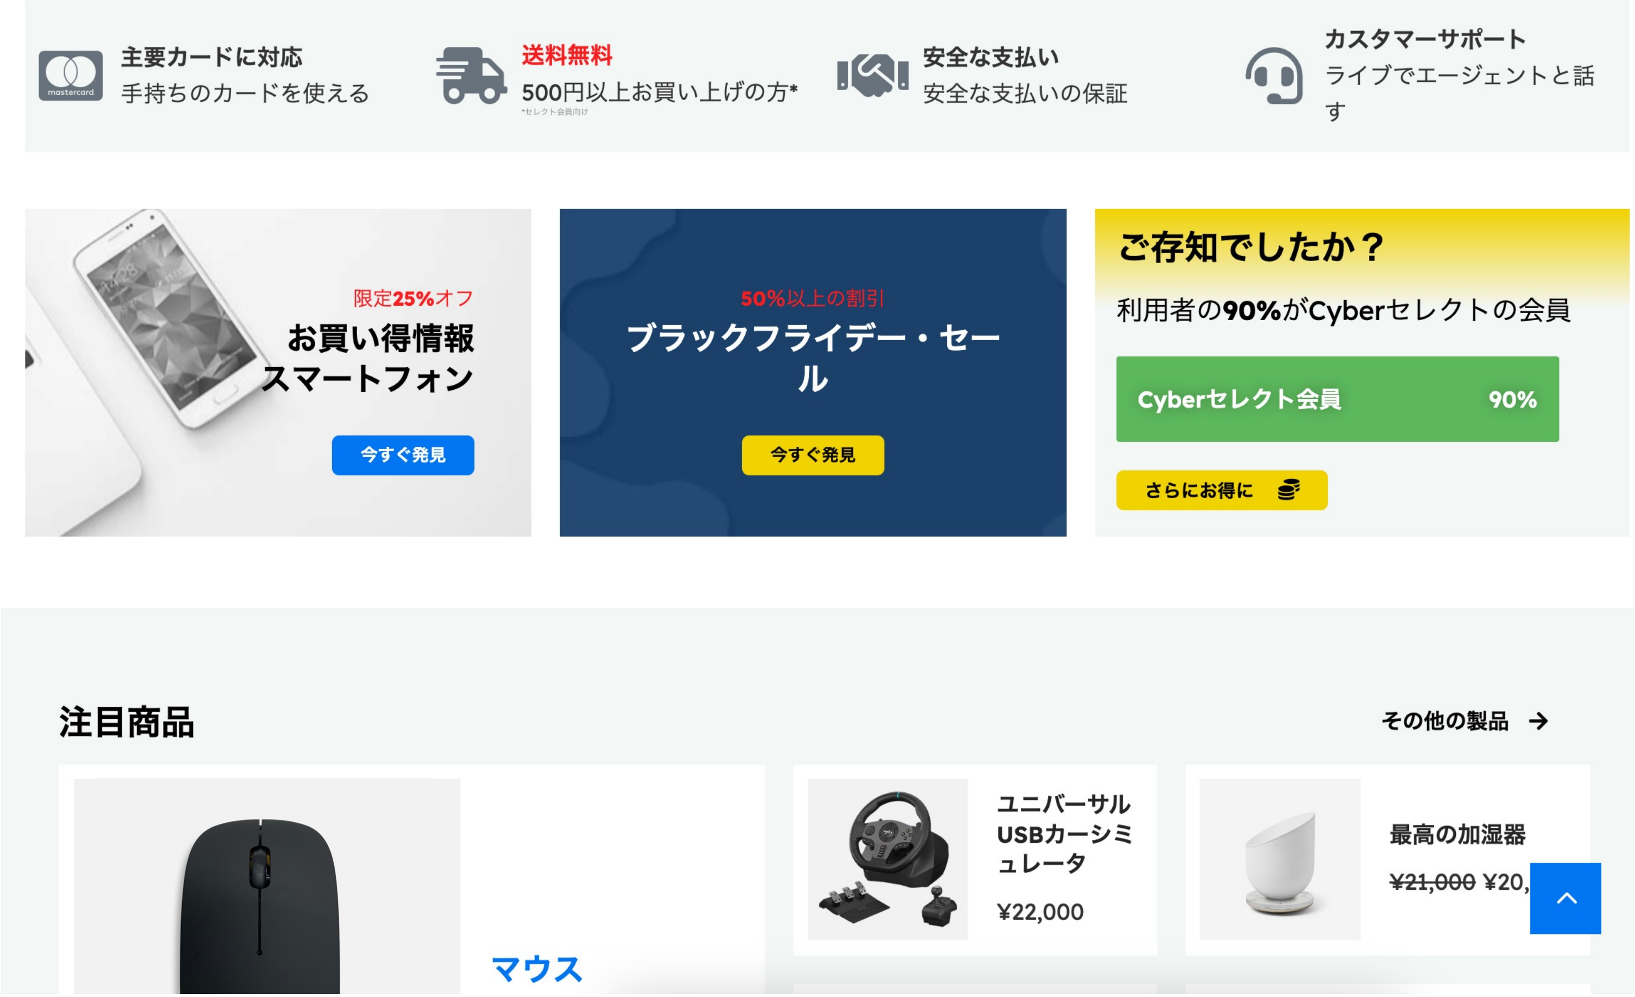

1

Browse the homepage

ホームページを見る

**Interface Interference**
Hidden Information
False Hierarchy
Toying with Emotions

**Social Proof**
Notification of Others' Activities

**Urgency**
Countdown Timer

**Nagging**
Membership Nagging

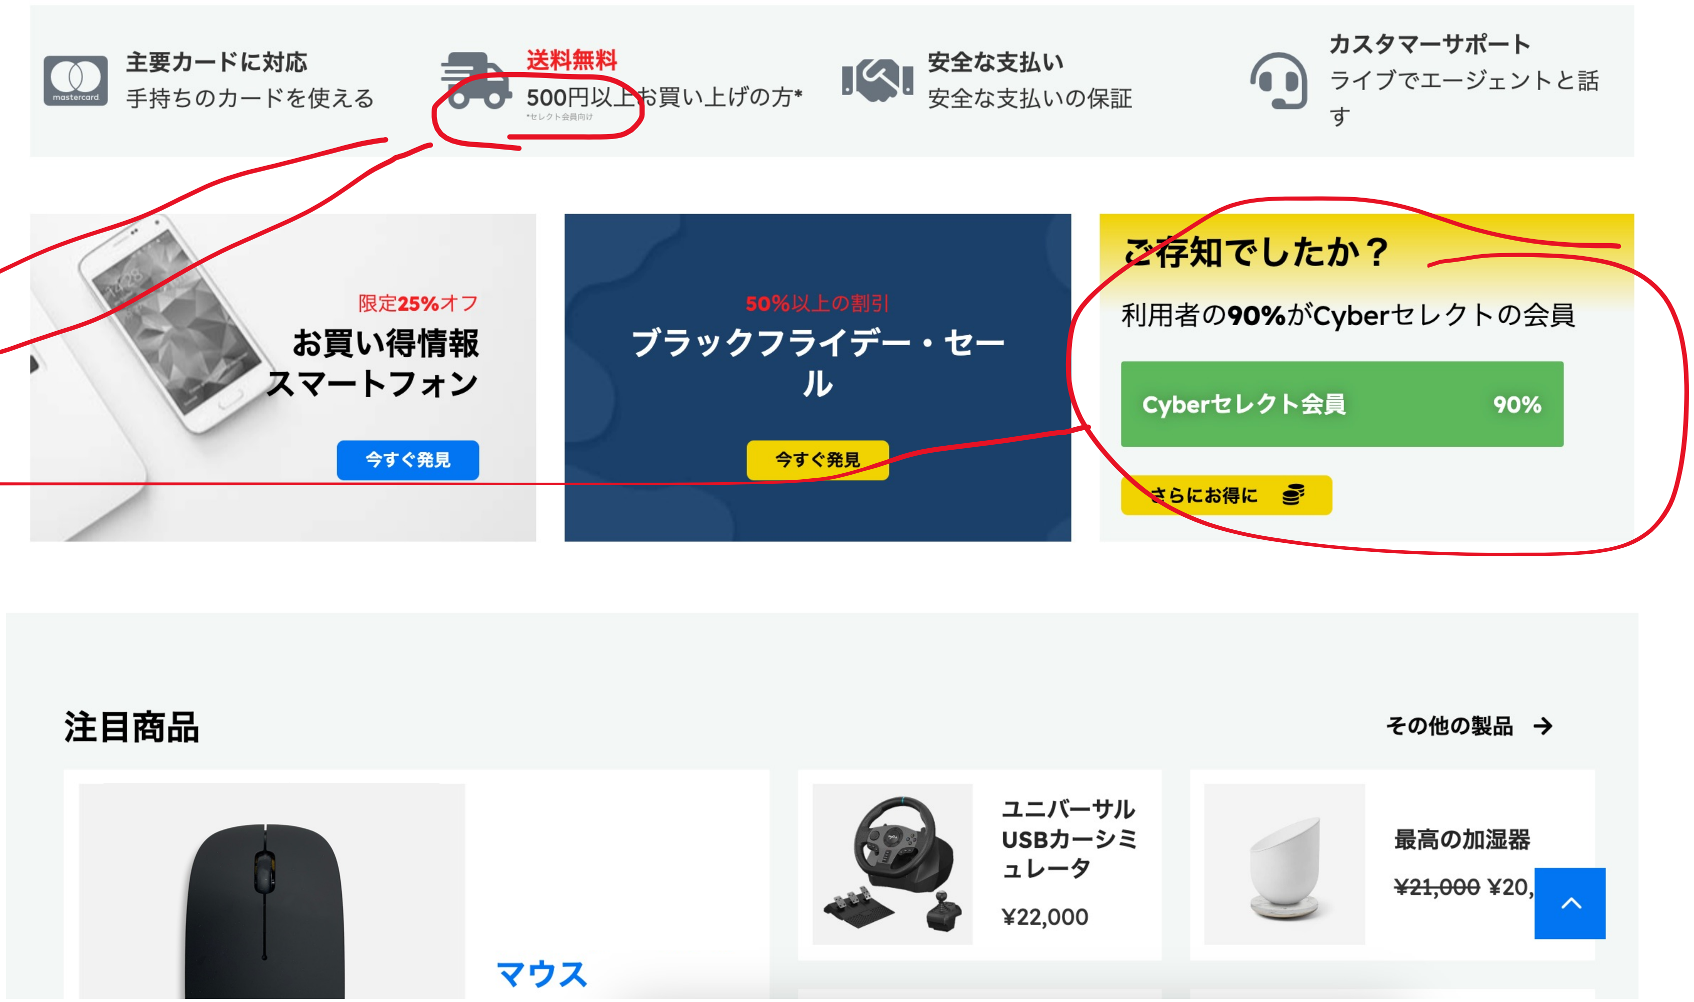

1

Browse the homepage

ホームページを見る

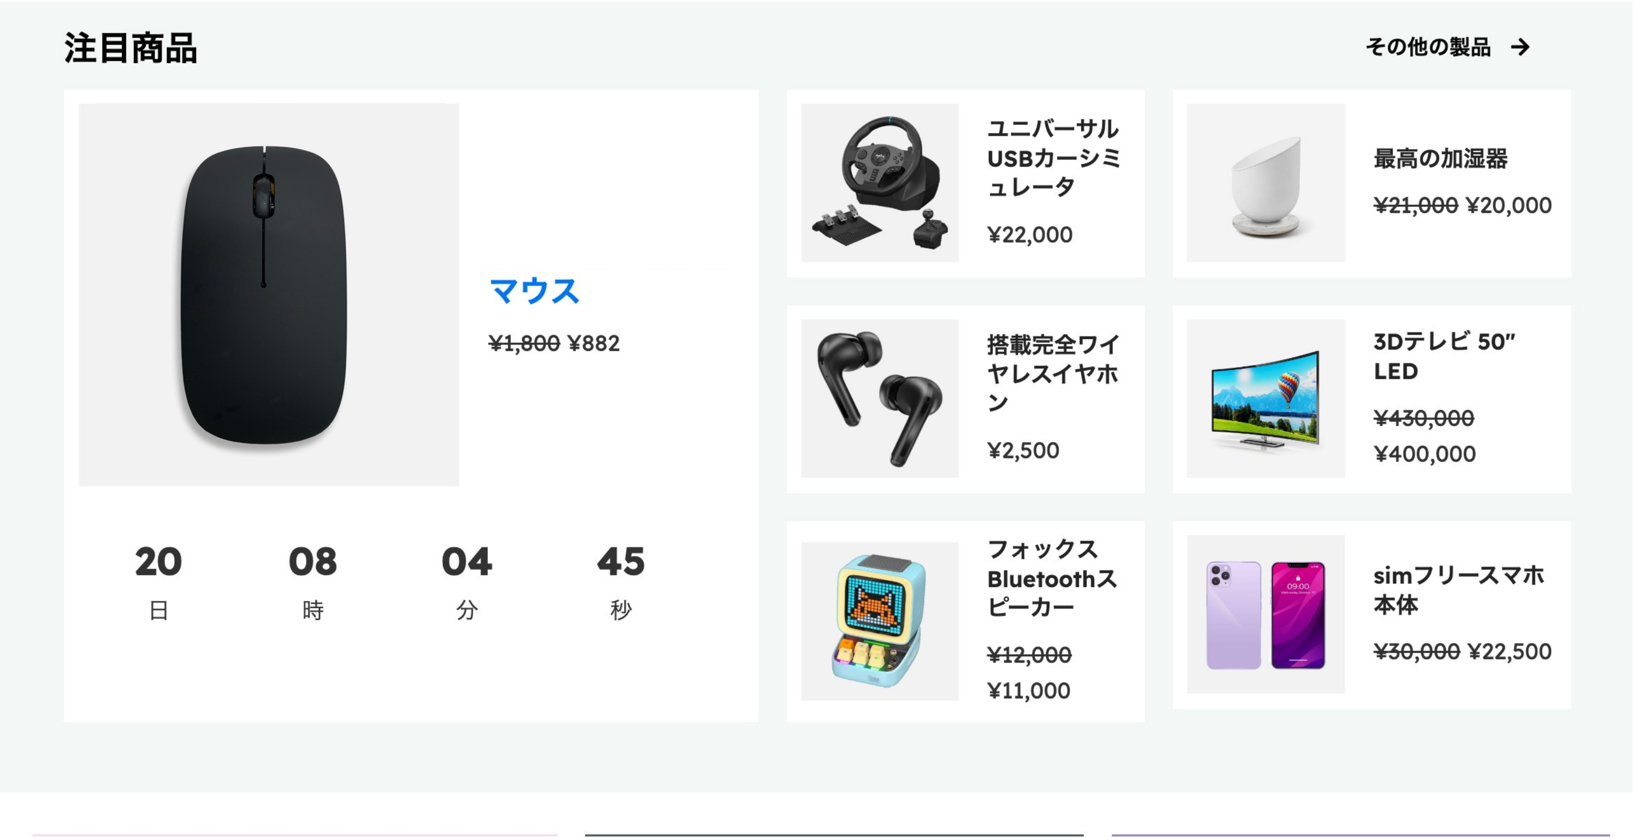

1

Browse the homepage

ホームページを見る

**Interface Interference**

Hidden Information

False Hierarchy

Toying with Emotions

**Social Proof**

Notification of Others' Activities

**Urgency**

Countdown Timer

**Nagging**

Membership Nagging

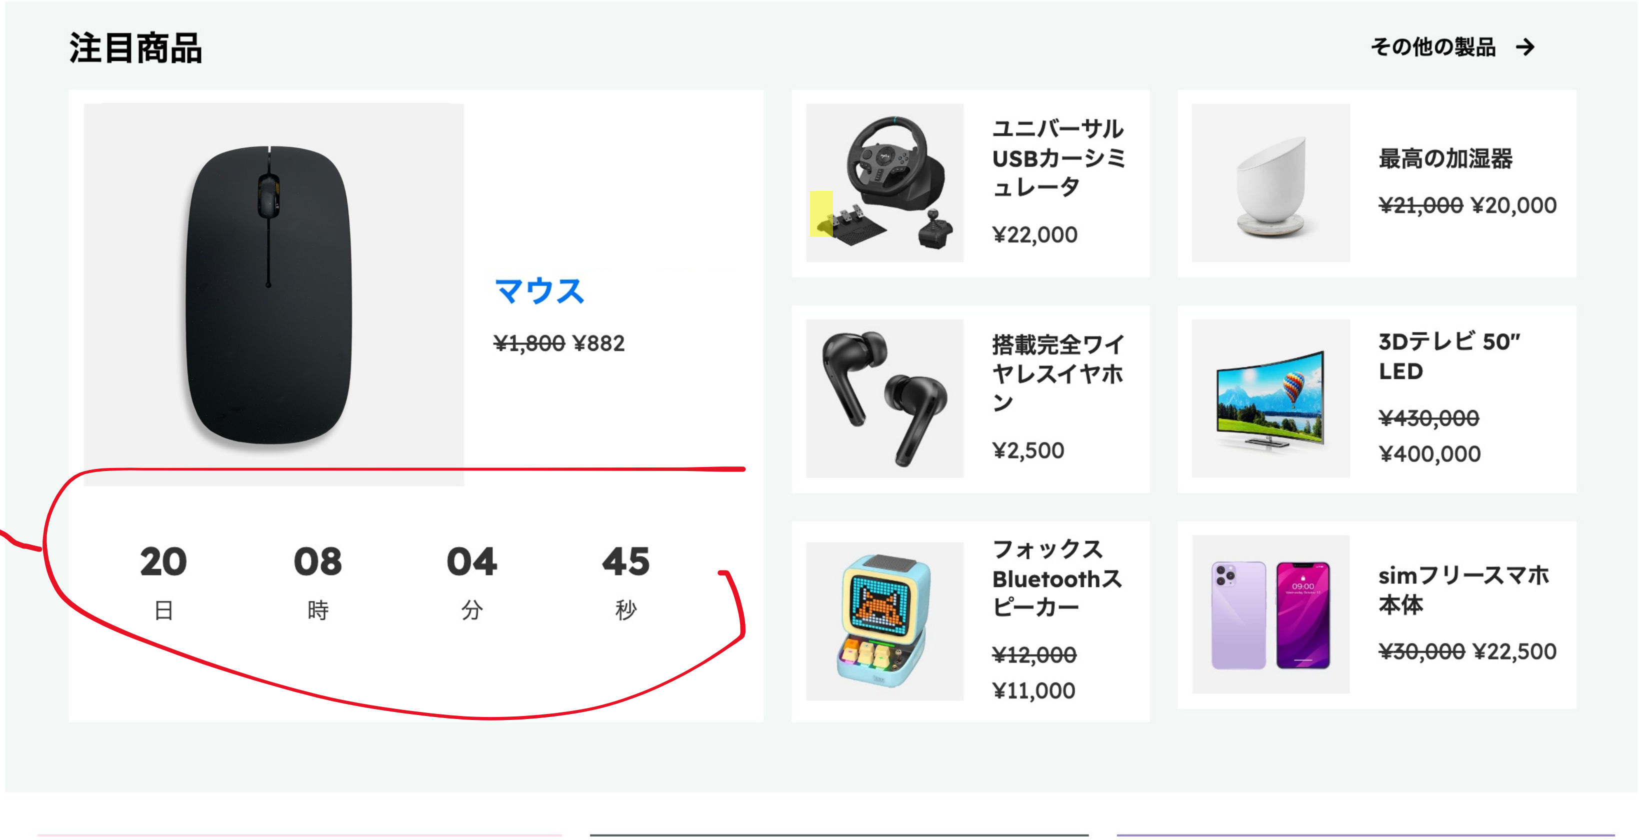

1

Browse the homepage

ホームページを見る

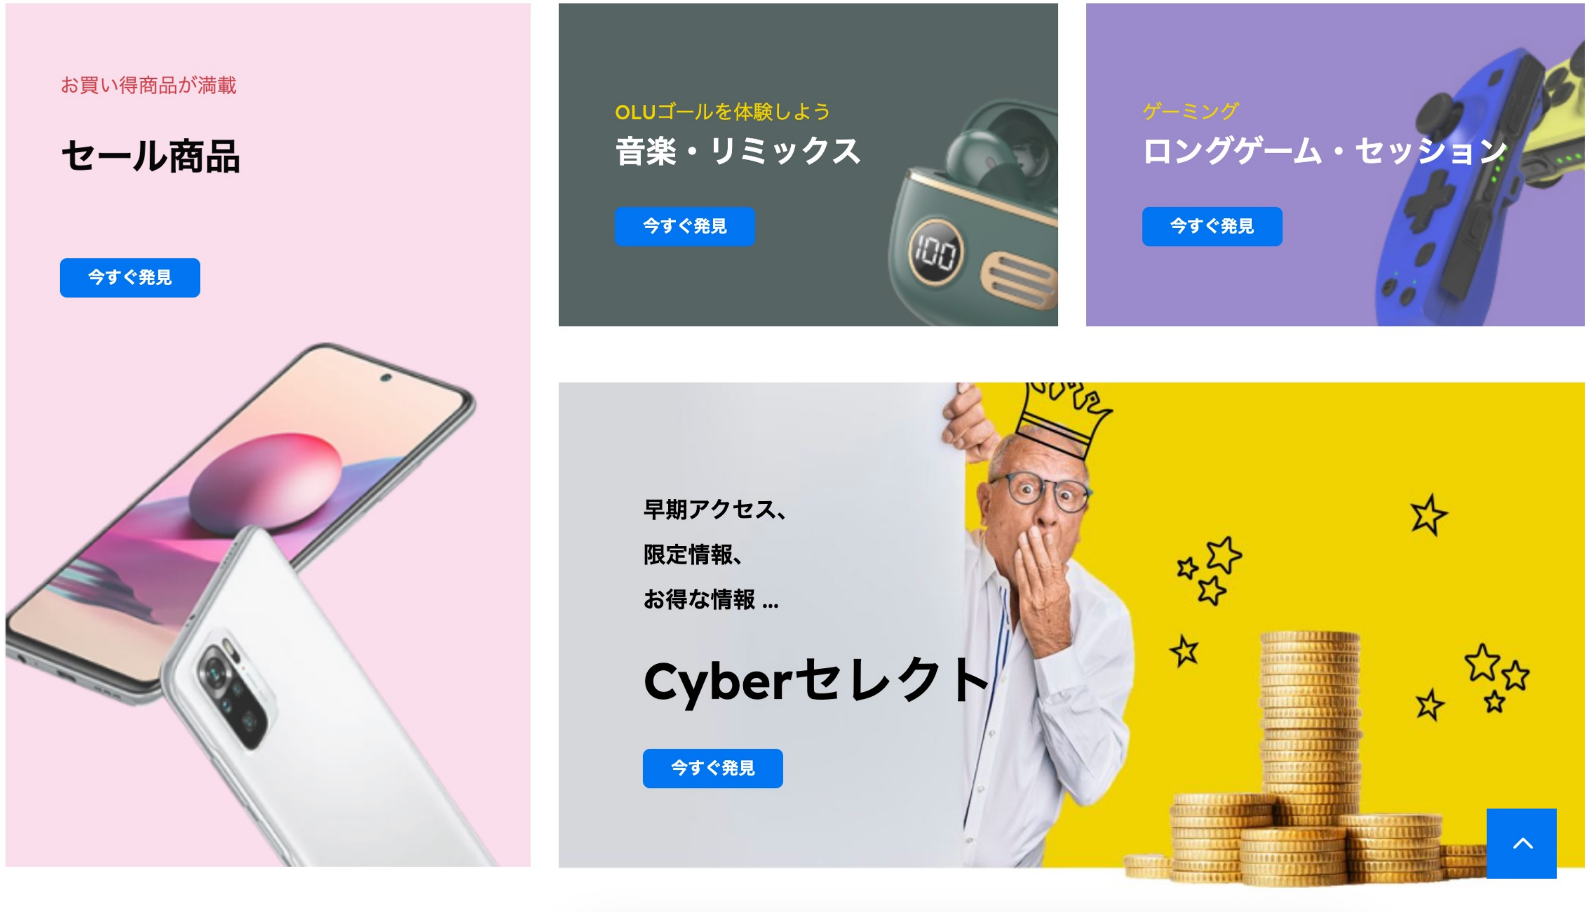

1

Browse the homepage

ホームページを見る

**Interface Interference**

Hidden Information

False Hierarchy

Toying with Emotions

**Social Proof**

Notification of Others’ Activities

**Urgency**

Countdown Timer

**Nagging**

Membership Nagging

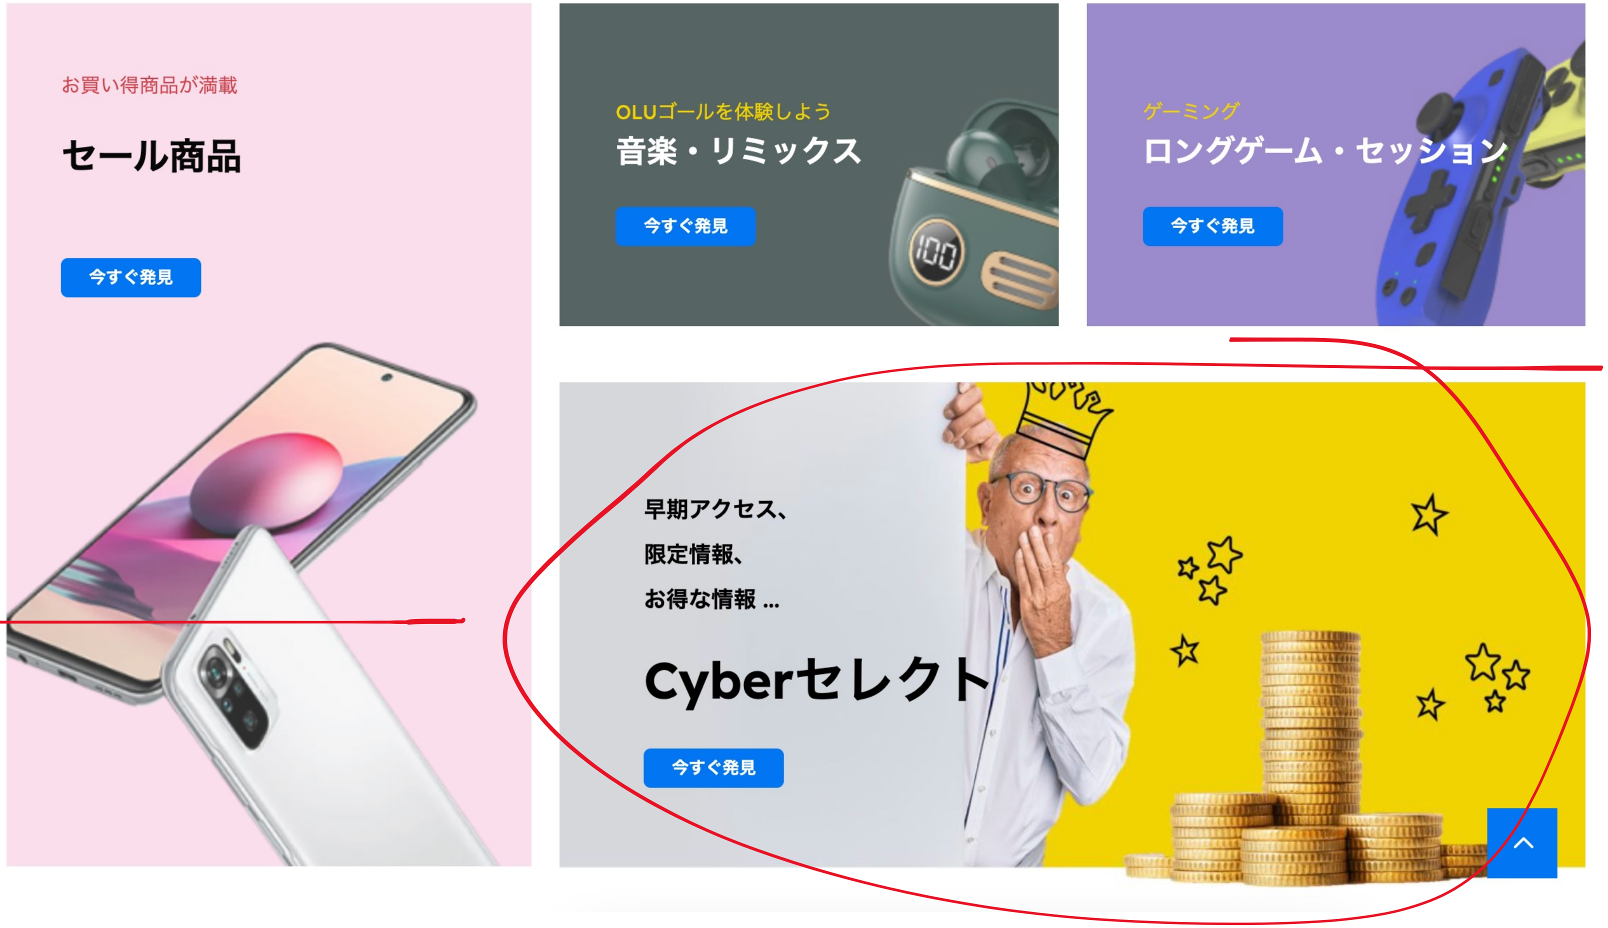

1

Browse the homepage

ホームページを見る

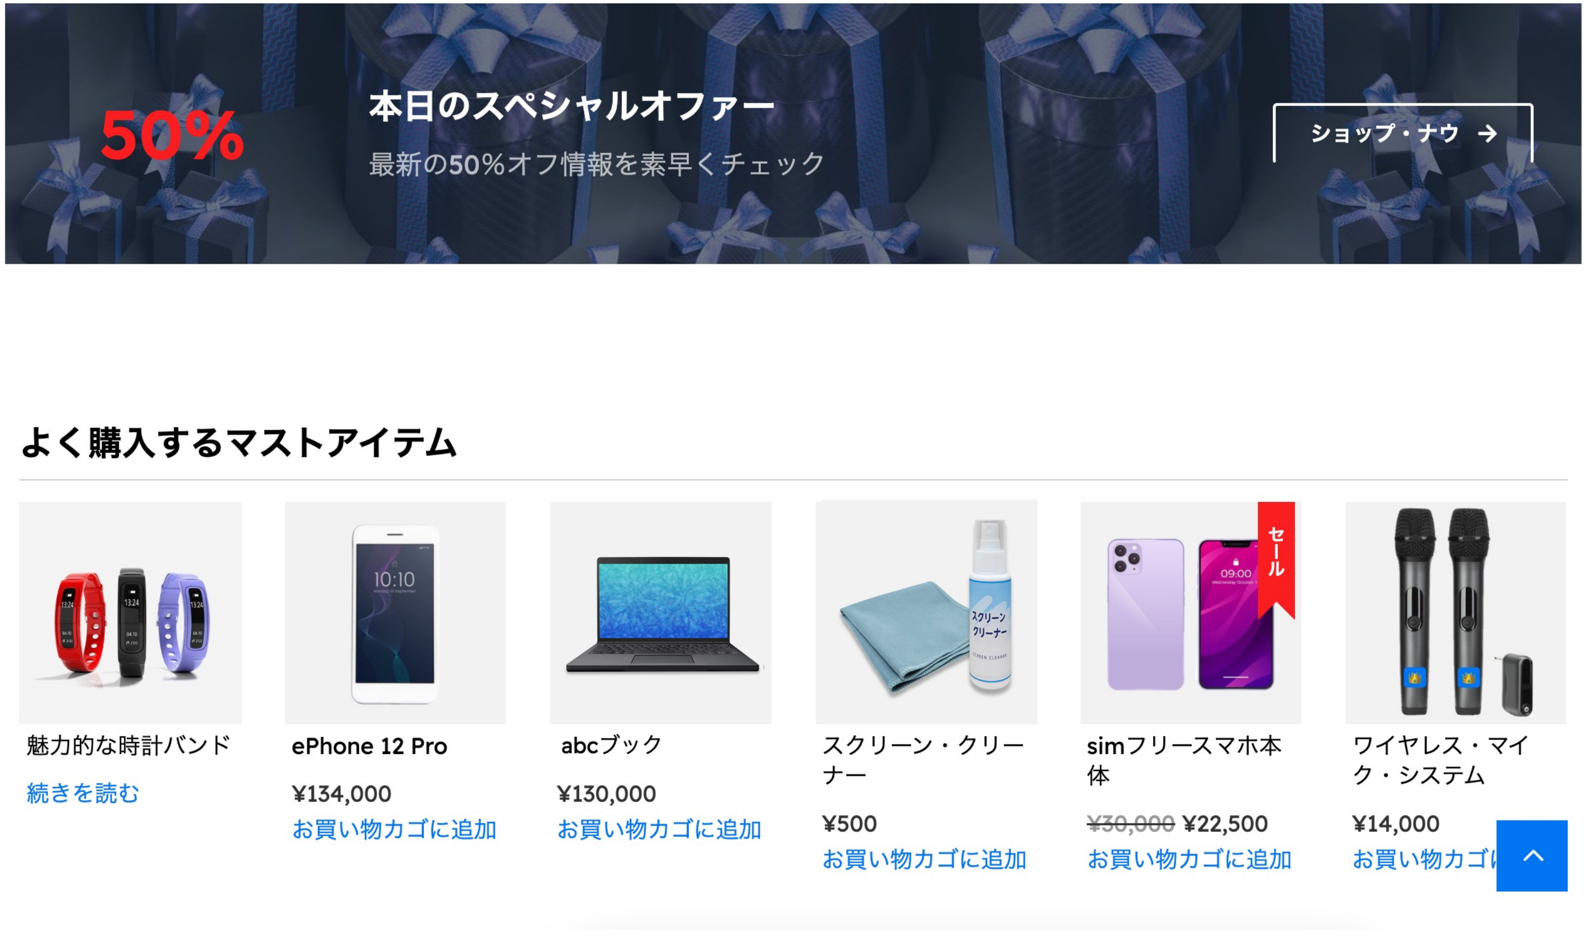

1

Browse the homepage

ホームページを見る

**Interface Interference**
Hidden Information
False Hierarchy
Toying with Emotions

**Social Proof**
Notification of Others' Activities

**Urgency**
Countdown Timer

**Nagging**
Membership Nagging

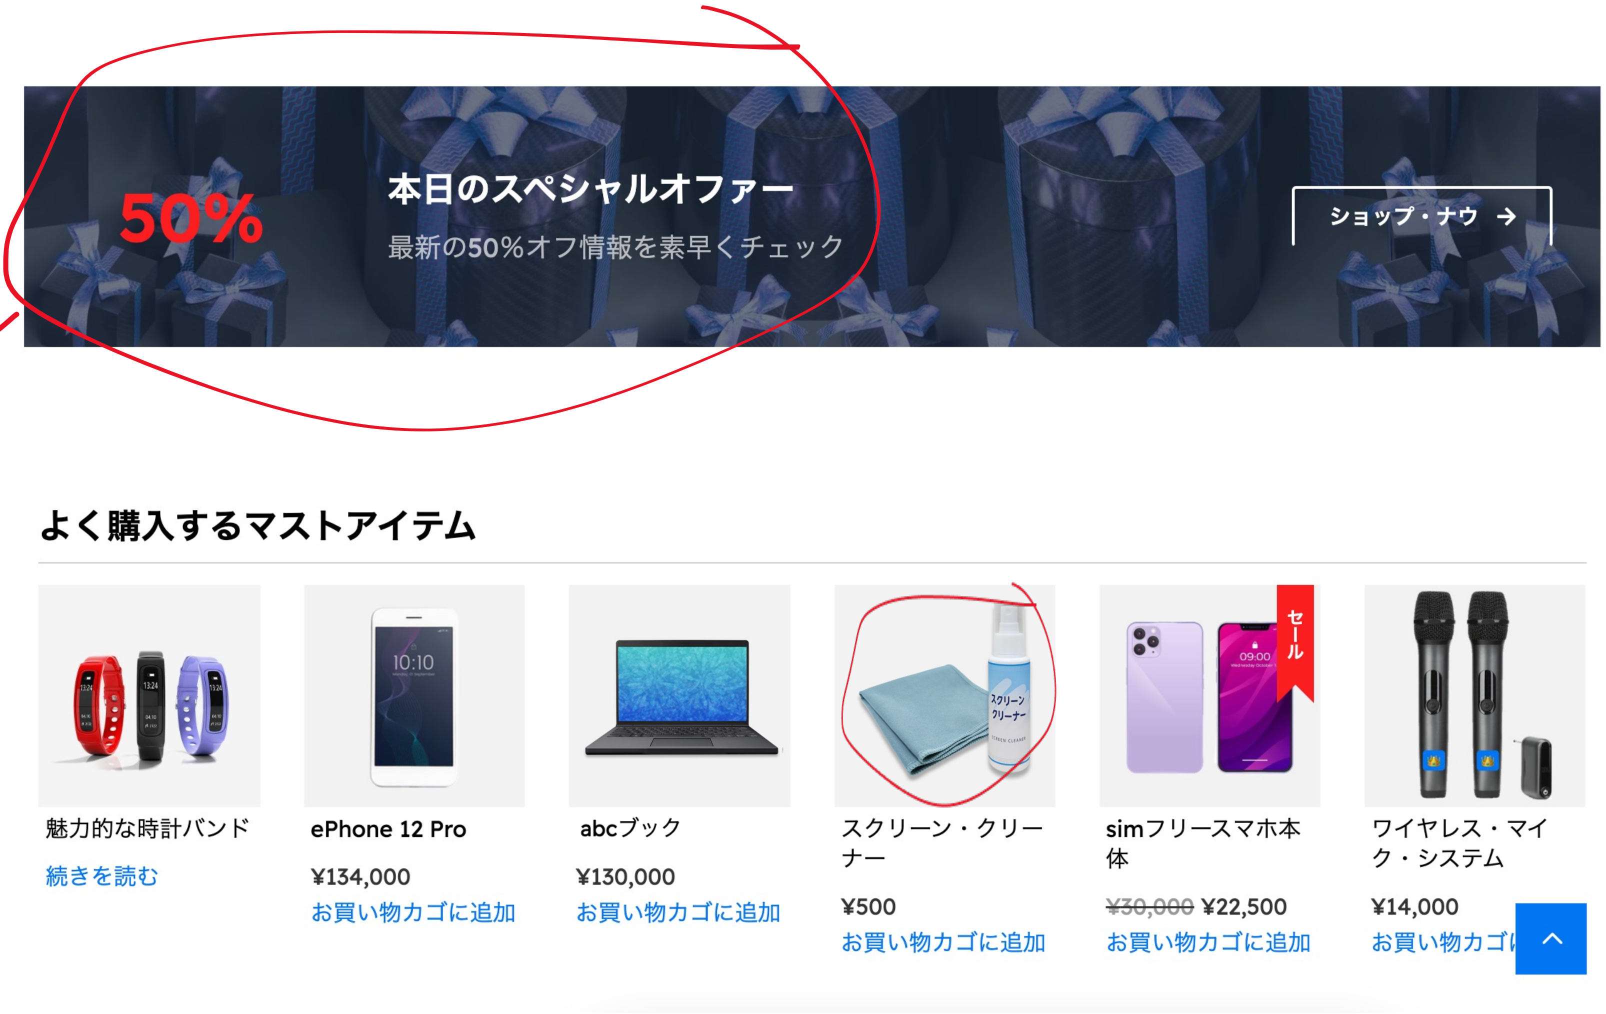

2

Browse for a set of items

ショップでセットを作る

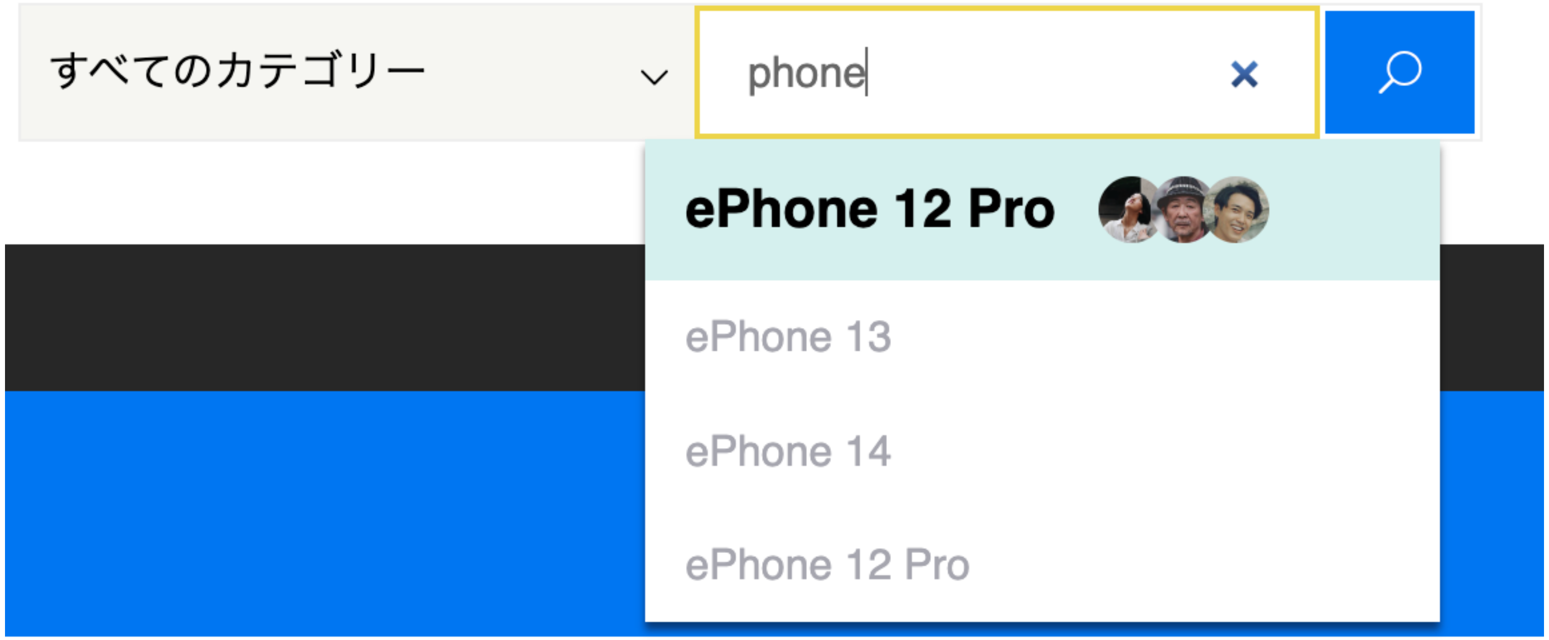

2

Browse for a set of items

ショップでセットを作る

**Interface Interference**

Preselection

False Hierarchy

**Social Proof**

Notification of Others' Activities

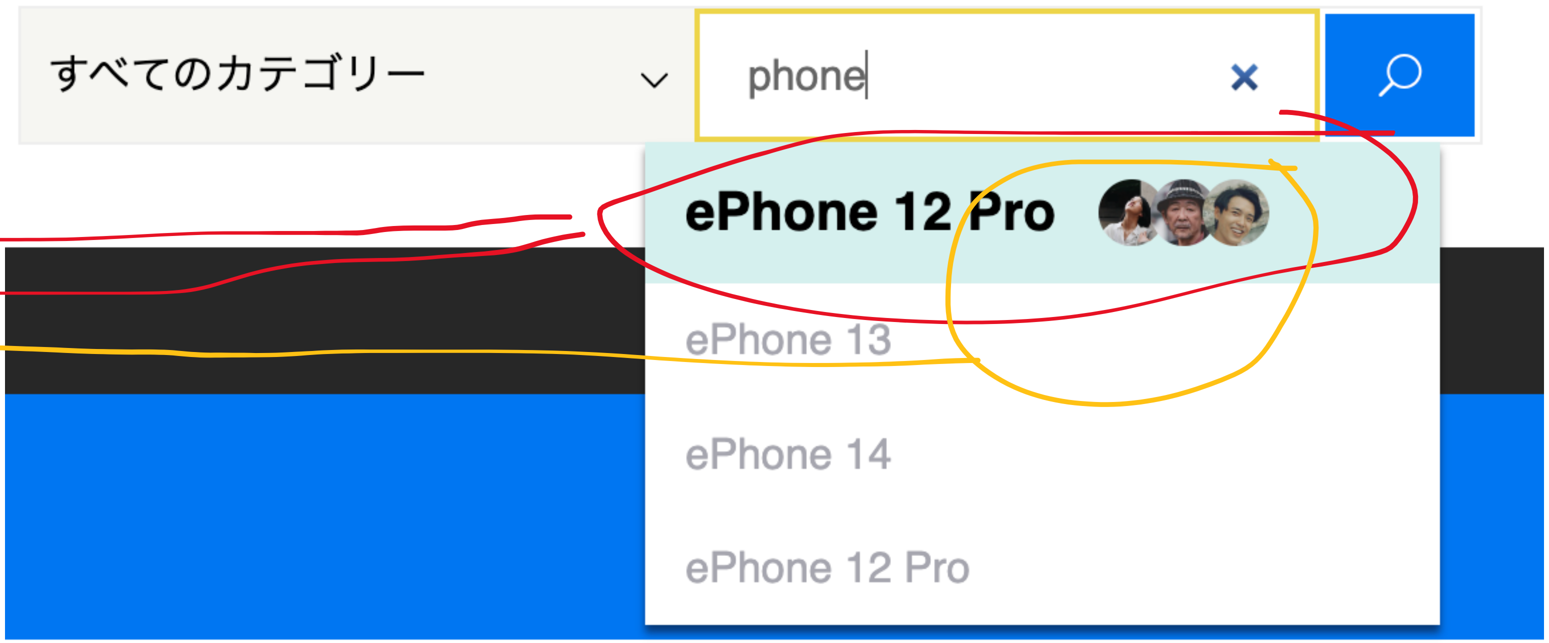

2

Browse for a set of items

ショップでセットを作る

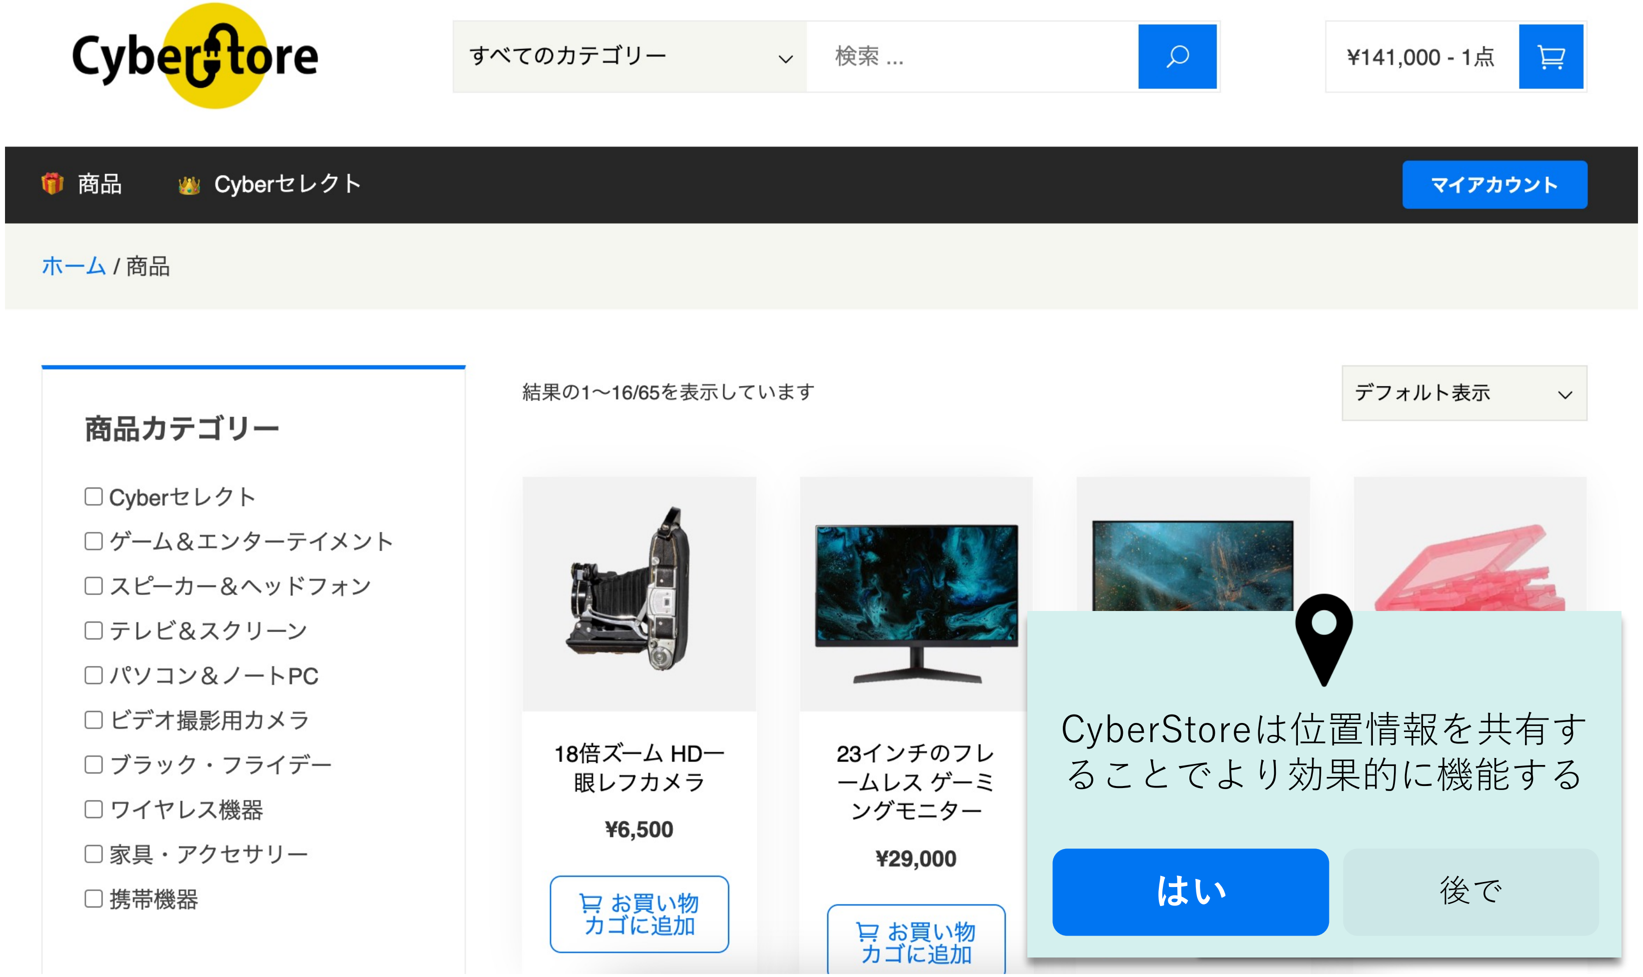

2

Browse for a set of items

ショップでセットを作る

**Nagging**

Turn On Location-Tracking

**Interface Interference**

False Hierarchy

Toying with Emotions

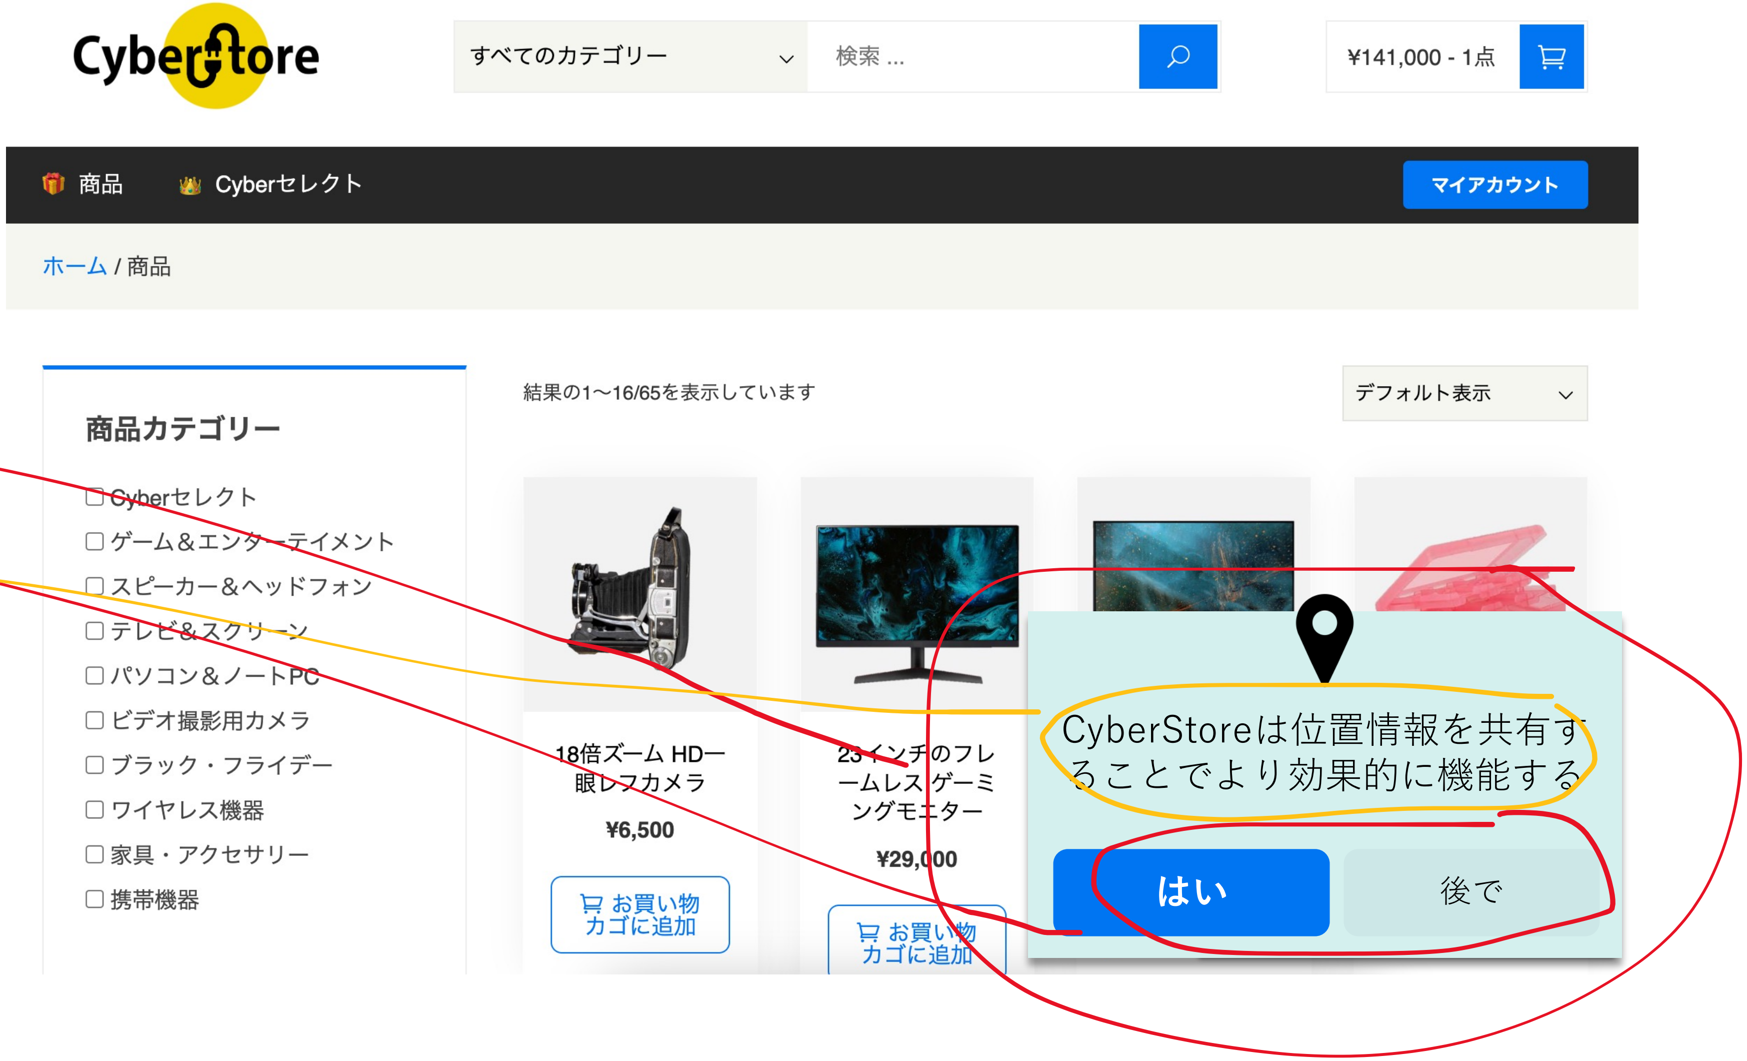

2

Browse for a set of items

ショップでセットを作る

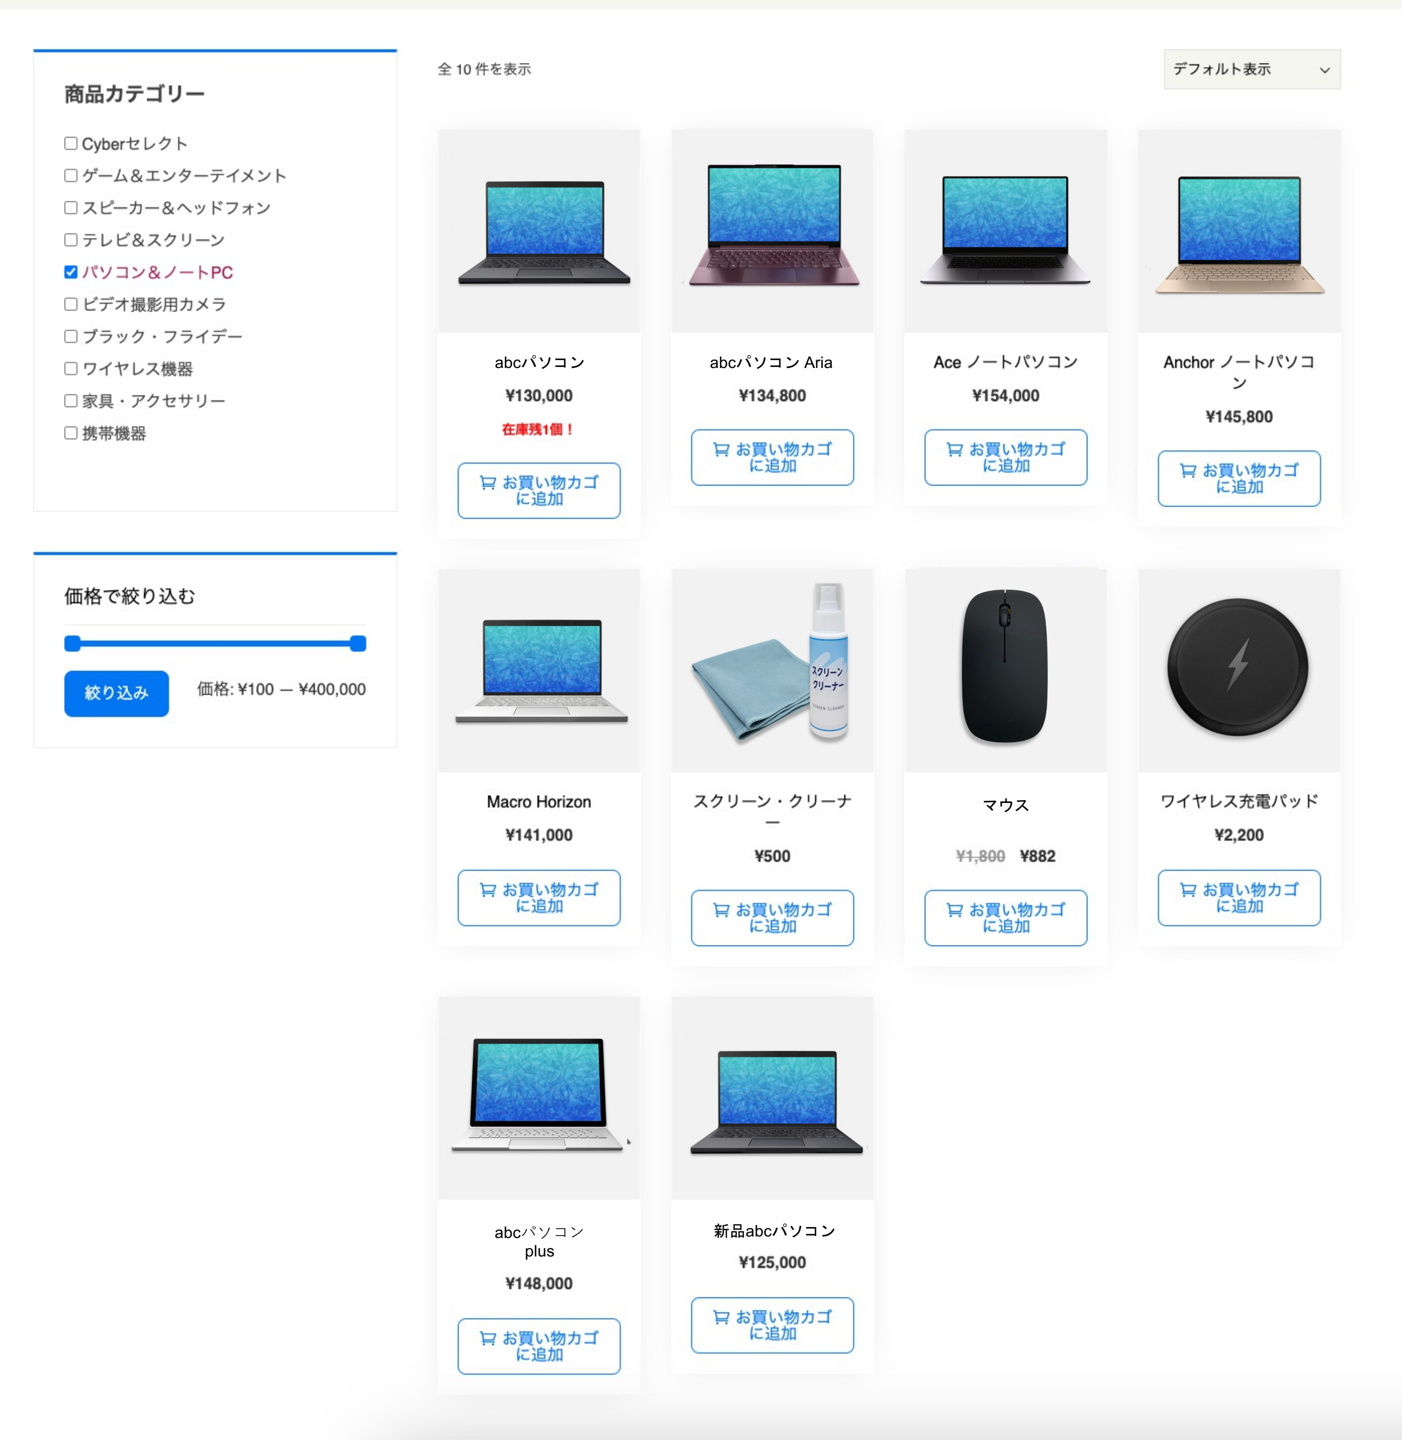

2

Browse for a set of items

ショップでセットを作る

**Interface Interference**

False Hierarchy

Toying with Emotions

Misleading Reference Pricing

**Urgency**

Low Stock/High Demand

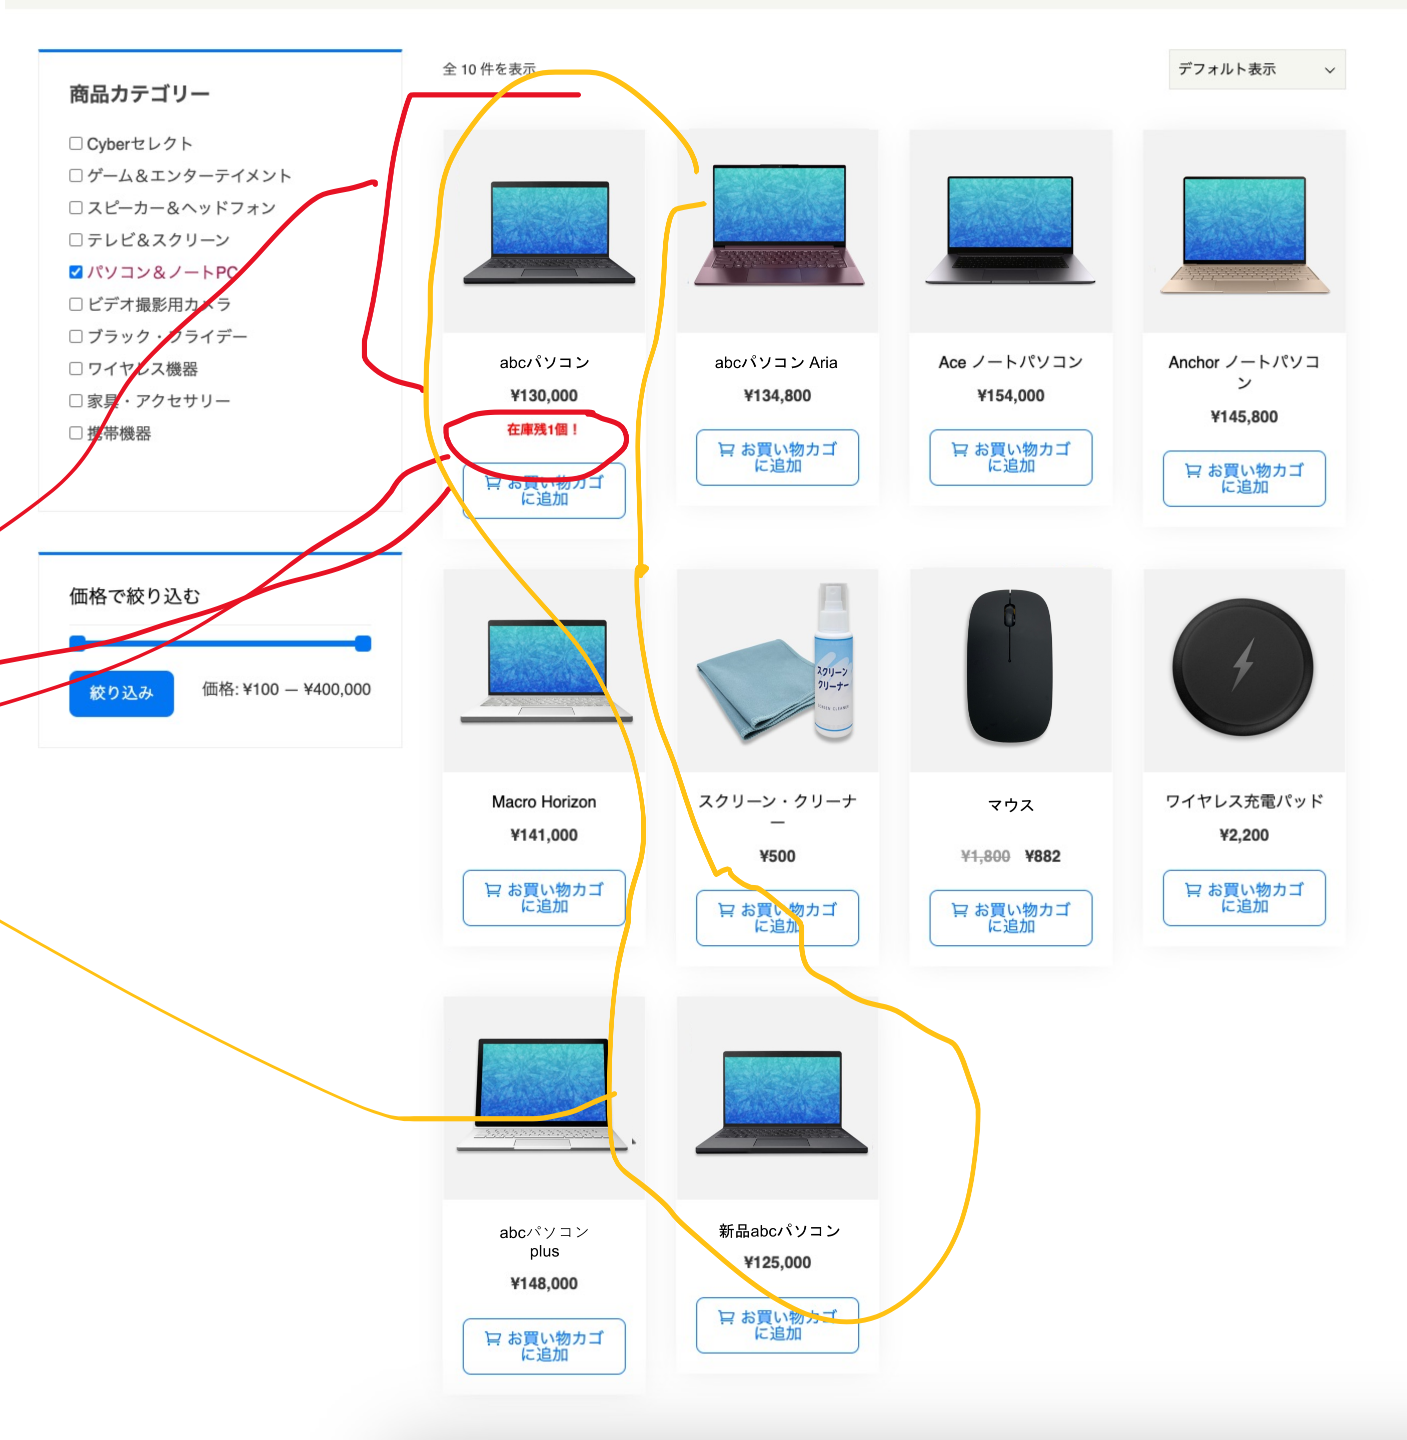

2

Browse for a set of items

ショップでセットを作る

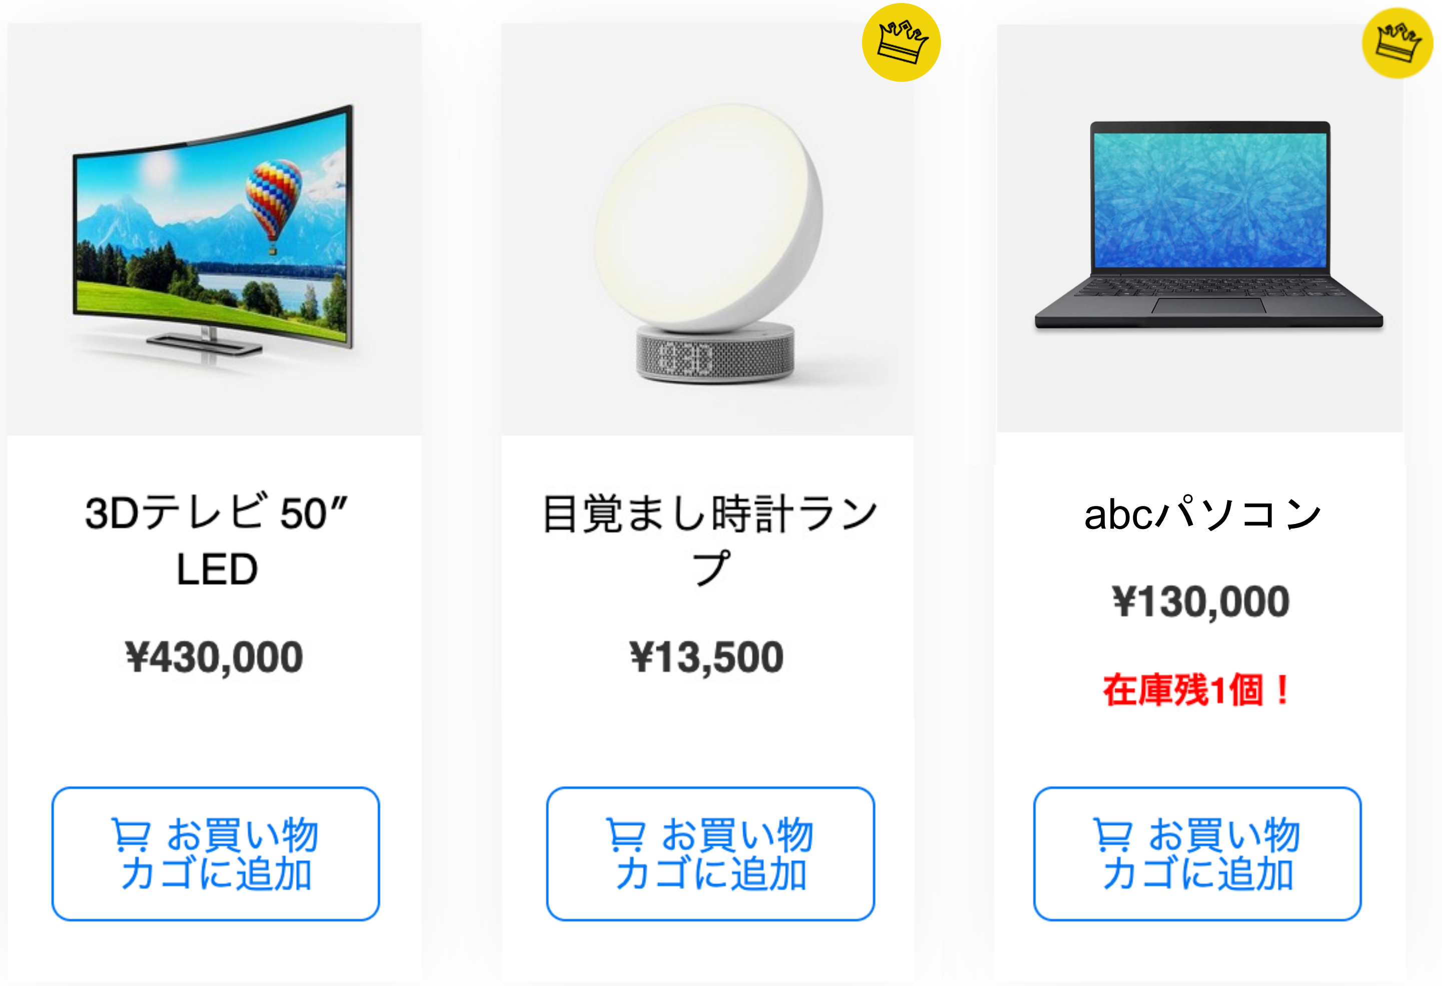

2

Browse for a set of items

ショップでセットを作る

**Urgency**

Low Stock/High Demand

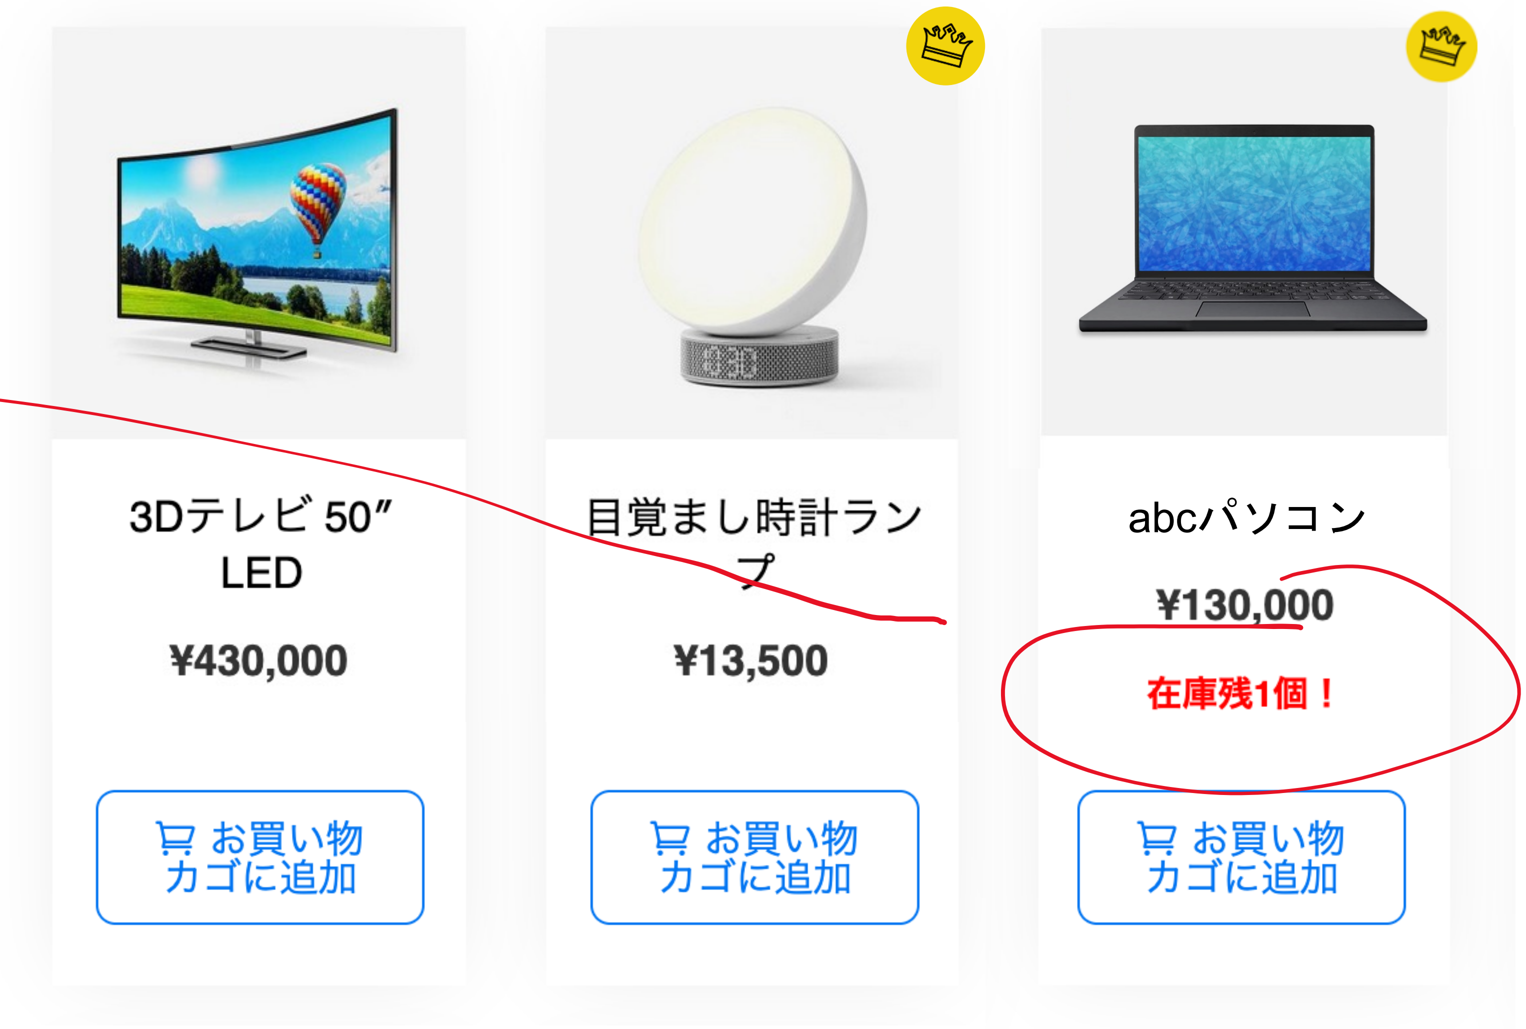

2

Browse for a set of items

ショップでセットを作る

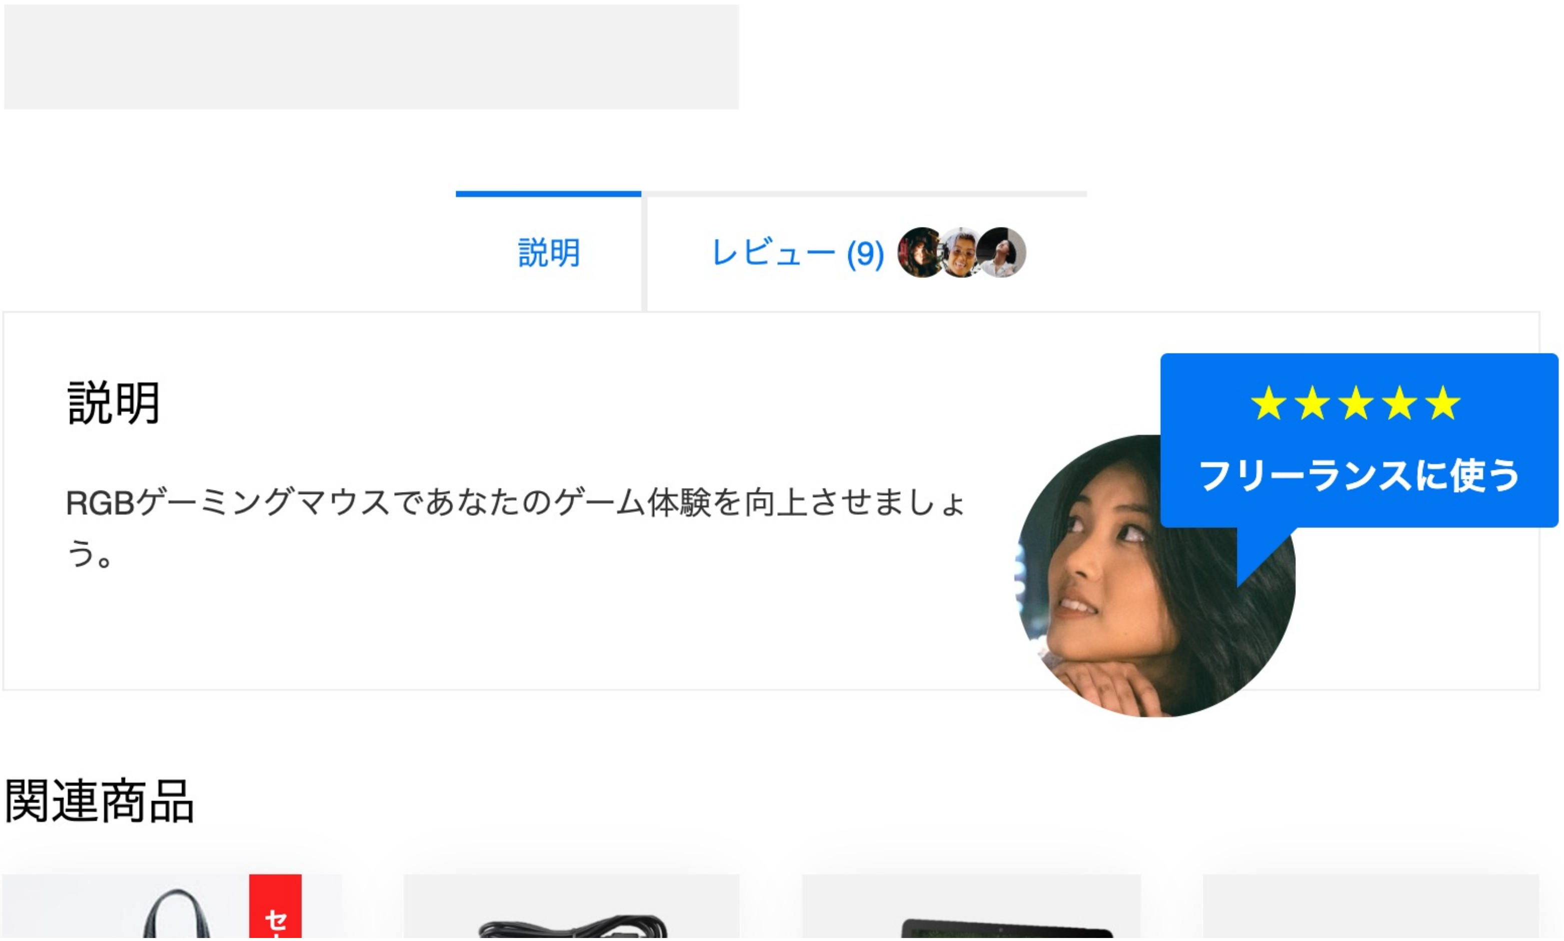

2

Browse for a set of items

ショップでセットを作る

**Social Proof**

Testimonials

Notification of Others' Activities

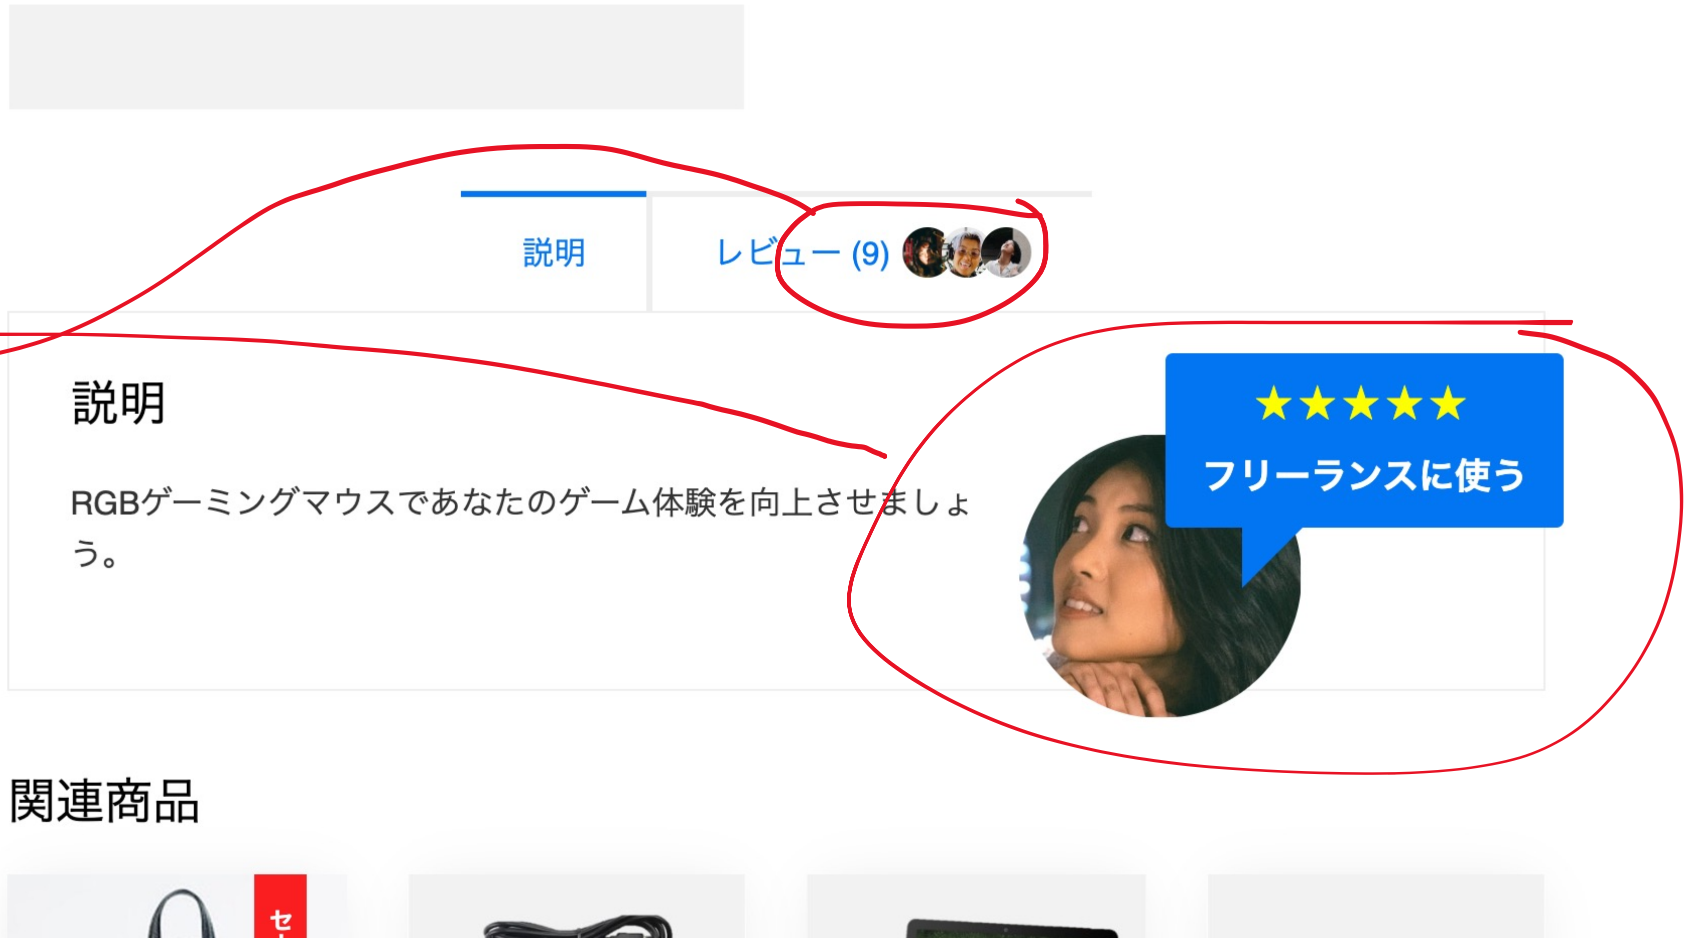

2

Browse for a set of items

ショップでセットを作る

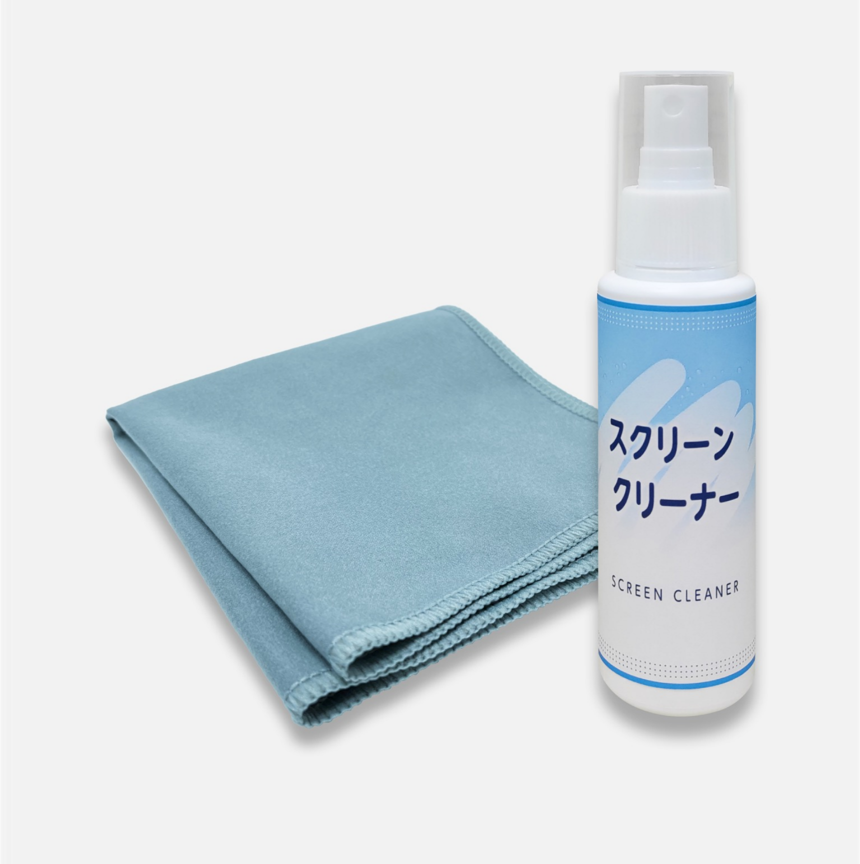


## スクリーン・クリーナー

☐ 購入は1回限り

￥500

☑ お得な月額プラン
毎月10%割引

￥450

在庫あり

数量: 1

選択

2

Browse for a set of items

ショップでセットを作る

**Interface Interference**

Preselection

False Hierarchy

Hidden Information

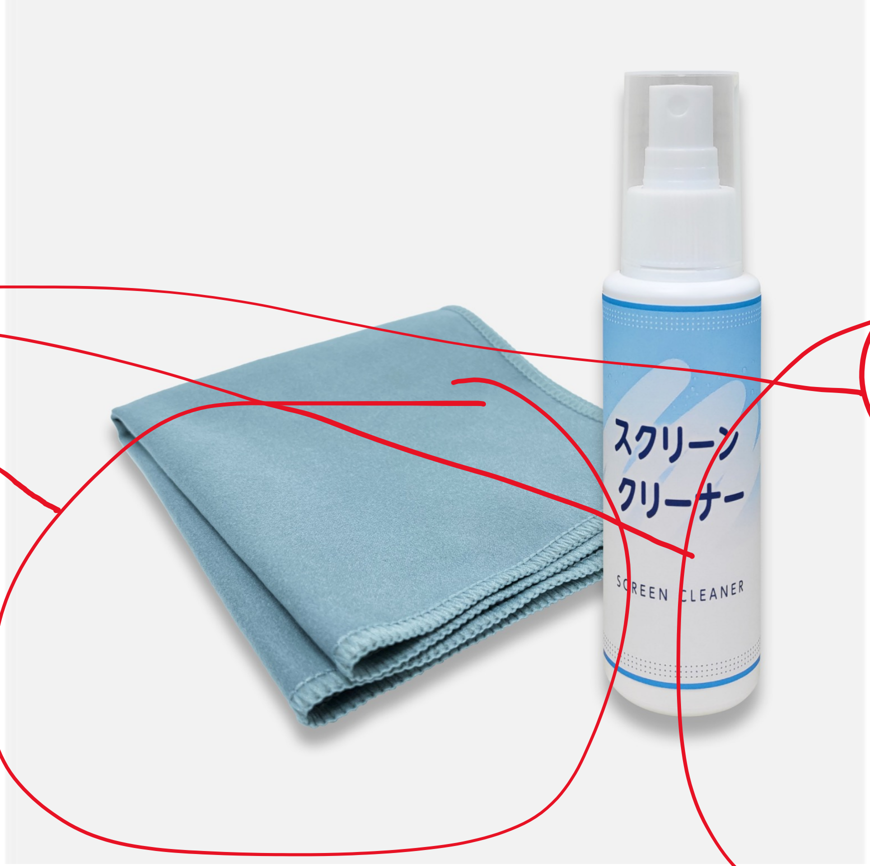


## スクリーン・クリーナー

☐ 購入は1回限り

￥500

☑ お得な月額プラン

毎月10%割引

￥450

在庫あり

数量: 1

選択

2

Browse for a set of items

ショップでセットを作る

| | 商品 | 数量 | 小計 | |
|---|---|---|---|---|
| 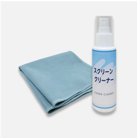 | サブスクリプション<br>スクリーン・クリーナー<br>~~¥500~~ ¥450 | 1 | ¥450 | × |
| 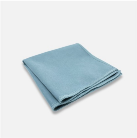 | マイクロファイバークロス<br>¥100 | 1 | ¥100 | × |



カートの更新

⏳ **6分41秒**の購入で**当日配達**

## お買い物カゴの合計

| | |
|---|---|
| **小計** | ¥550 |
| **配送** | 定額送料<br>**東京都 東京工業大学** に配送します。<br>住所を変更 |
| **販売手数料** | ¥350 |
| **合計** | **¥900** |

購入手続きに進む

2

Browse for a set of items

ショップでセットを作る

**Sneaking**

Sneaking an Item

**Urgency**

Countdown Timer

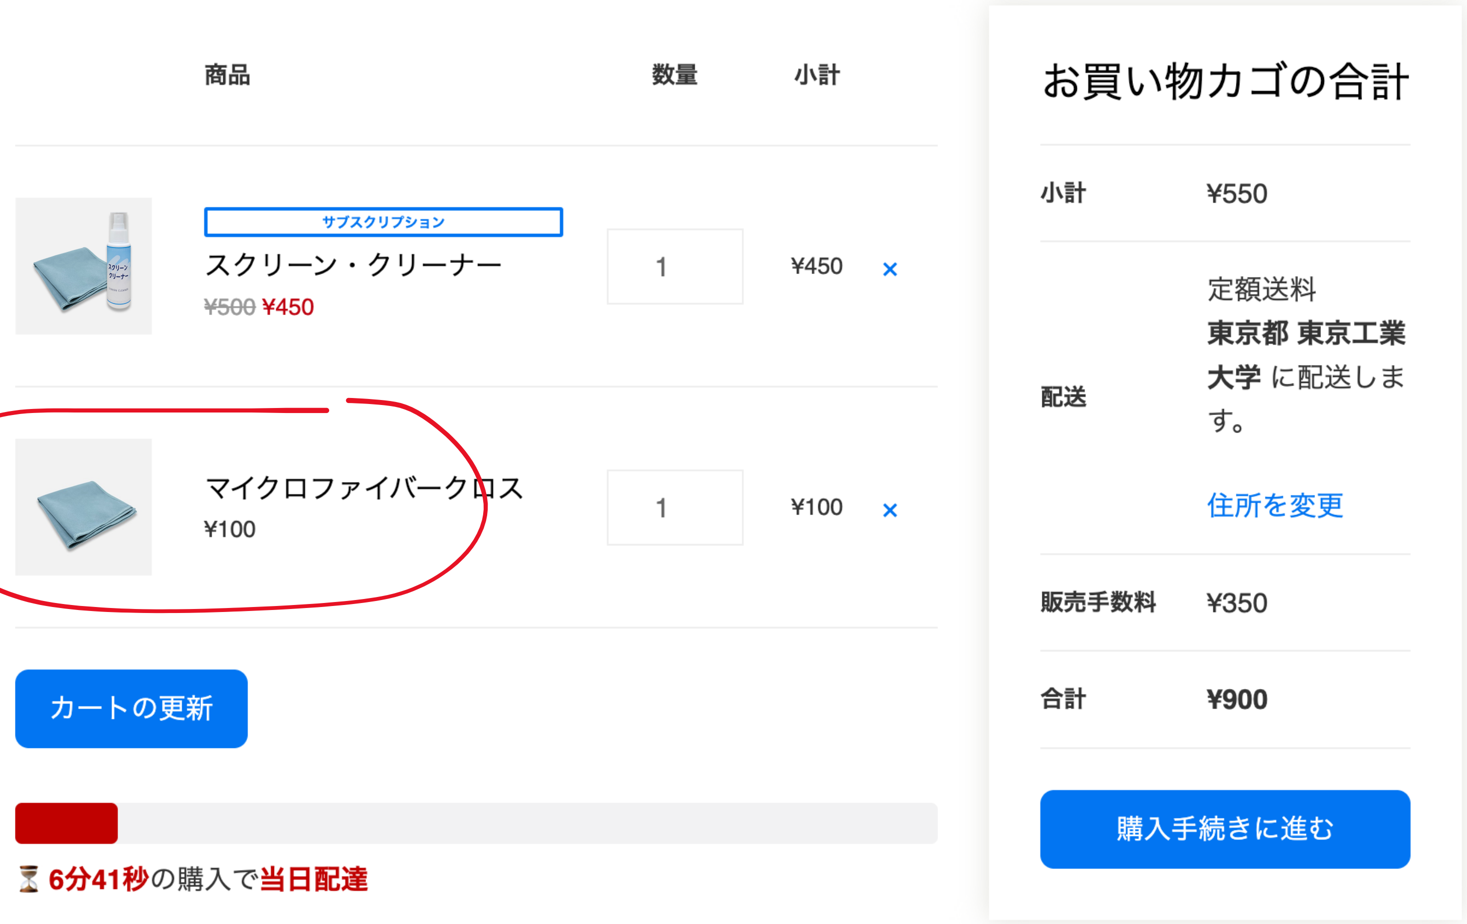

3

Check-out and sign up

チェックアウトとサインアップ

# CyberStoreに参加する

名前

メール

パスワード

**サインアップ**

✓ 私は規約を読み、理解しました。

詳細はこちら▼

✓ 私は規約を読み、理解しました。

**閉じる**▲

✓ 電子メールを送信することにより、当社および当社のパートナーからの電子メールおよび限定オファーの受信に同意したものとみなされます。詳しくは、**利用条件**をご覧ください。

3

Check-out and sign up

チェックアウトとサインアップ

**Forced Action**

Forced to Register

**Interface Interference**

Preselection ×2

Hidden Information

# CyberStoreに参加する

名前

メール

パスワード

**サインアップ**

✓ 私は規約を読み、理解しました。

詳細はこちら▼

✓ 私は規約を読み、理解しました。

閉じる▲

✓ 電子メールを送信することにより、当社および当社のパートナーからの電子メールおよび限定オファーの受信に同意したものとみなされます。詳しくは、利用条件をご覧ください。

3

Check-out and sign up

チェックアウトとサインアップ

# チェックアウト

ご住所

注文に関する注意事項

☐ Cyberセレクトに登録しない場合は、チェックを入れてください

☐ お客様が興味を持ちそうな商品やサービスについてのCyberStoreからの連絡が不要な場合は、チェックを入れてください

ご注文

| 商品 | 小計 |
|---|---|
| スクリーン・クリーナー × 1 | ¥450 |
| マイクロファイバークロス × 1 | ¥100 |
| **小計** | ¥550 |
| **配送** | 定額送料 |
| **販売手数料** | ¥350 |
| **合計** | **¥900** |

代金引換

配達時に現金で支払う。

注文する

3

Check-out and sign up

チェックアウトとサインアップ

**Interface Interference**

Trick Questions

**Nagging**

Membership Nagging

**Sneaking**

Drip Pricing

Hidden Subscription

# チェックアウト

ご住所

注文に関する注意事項

Cyberセレクトに登録しない場合は、チェックを入れてください

お客様が興味を持ちそうな商品やサービスについてのCyberStoreからの連絡が不要な場合は、チェックを入れてください

ご注文

| 商品 | 小計 |
|---|---|
| スクリーン・クリーナー × 1 | ¥450 |
| マイクロファイバークロス × 1 | ¥100 |
| 小計 | ¥550 |
| 配送 | 定額送料 |
| 販売手数料 | ¥350 |
| 合計 | ¥900 |

代金引換

配達時に現金で支払う。

注文する

3

Check-out and sign up

チェックアウトとサインアップ

ご注文ありがとうございます。

ー会員制サービスへようこそー

# Cyberセレクト

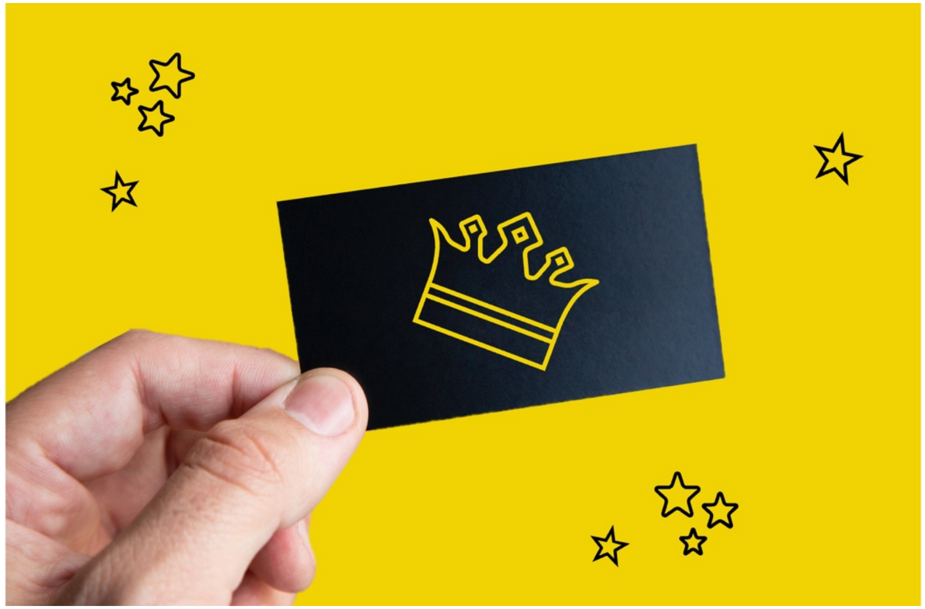

今すぐチェックしよう

3

Check-out and sign up

チェックアウトとサインアップ

**Nagging**
Membership Nagging

**Sneaking**
Hidden Subscription

ご注文ありがとうございます。

ー会員制サービスへようこそー

# Cyberセレクト

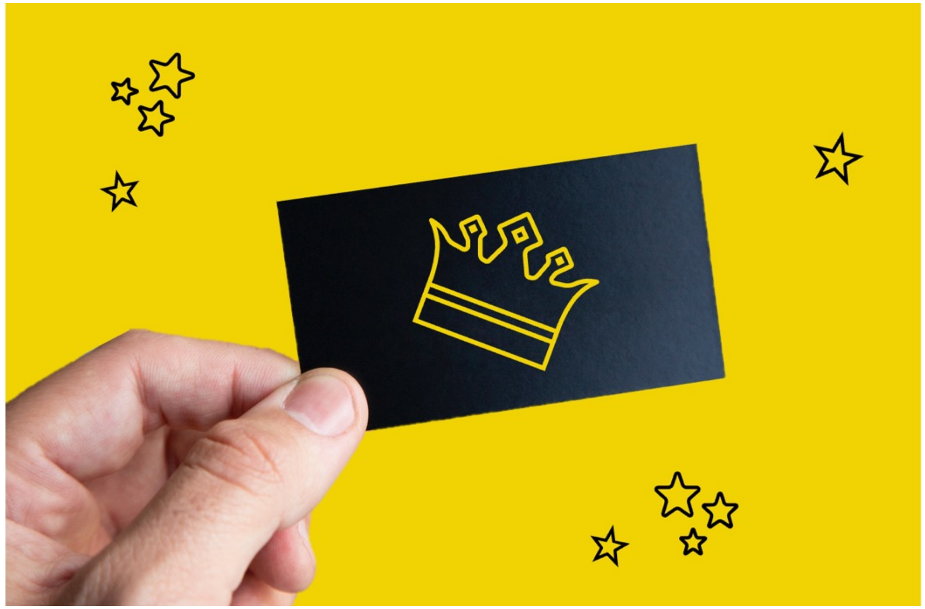

今すぐチェックしよう

3

Check-out and sign up

チェックアウトとサインアップ

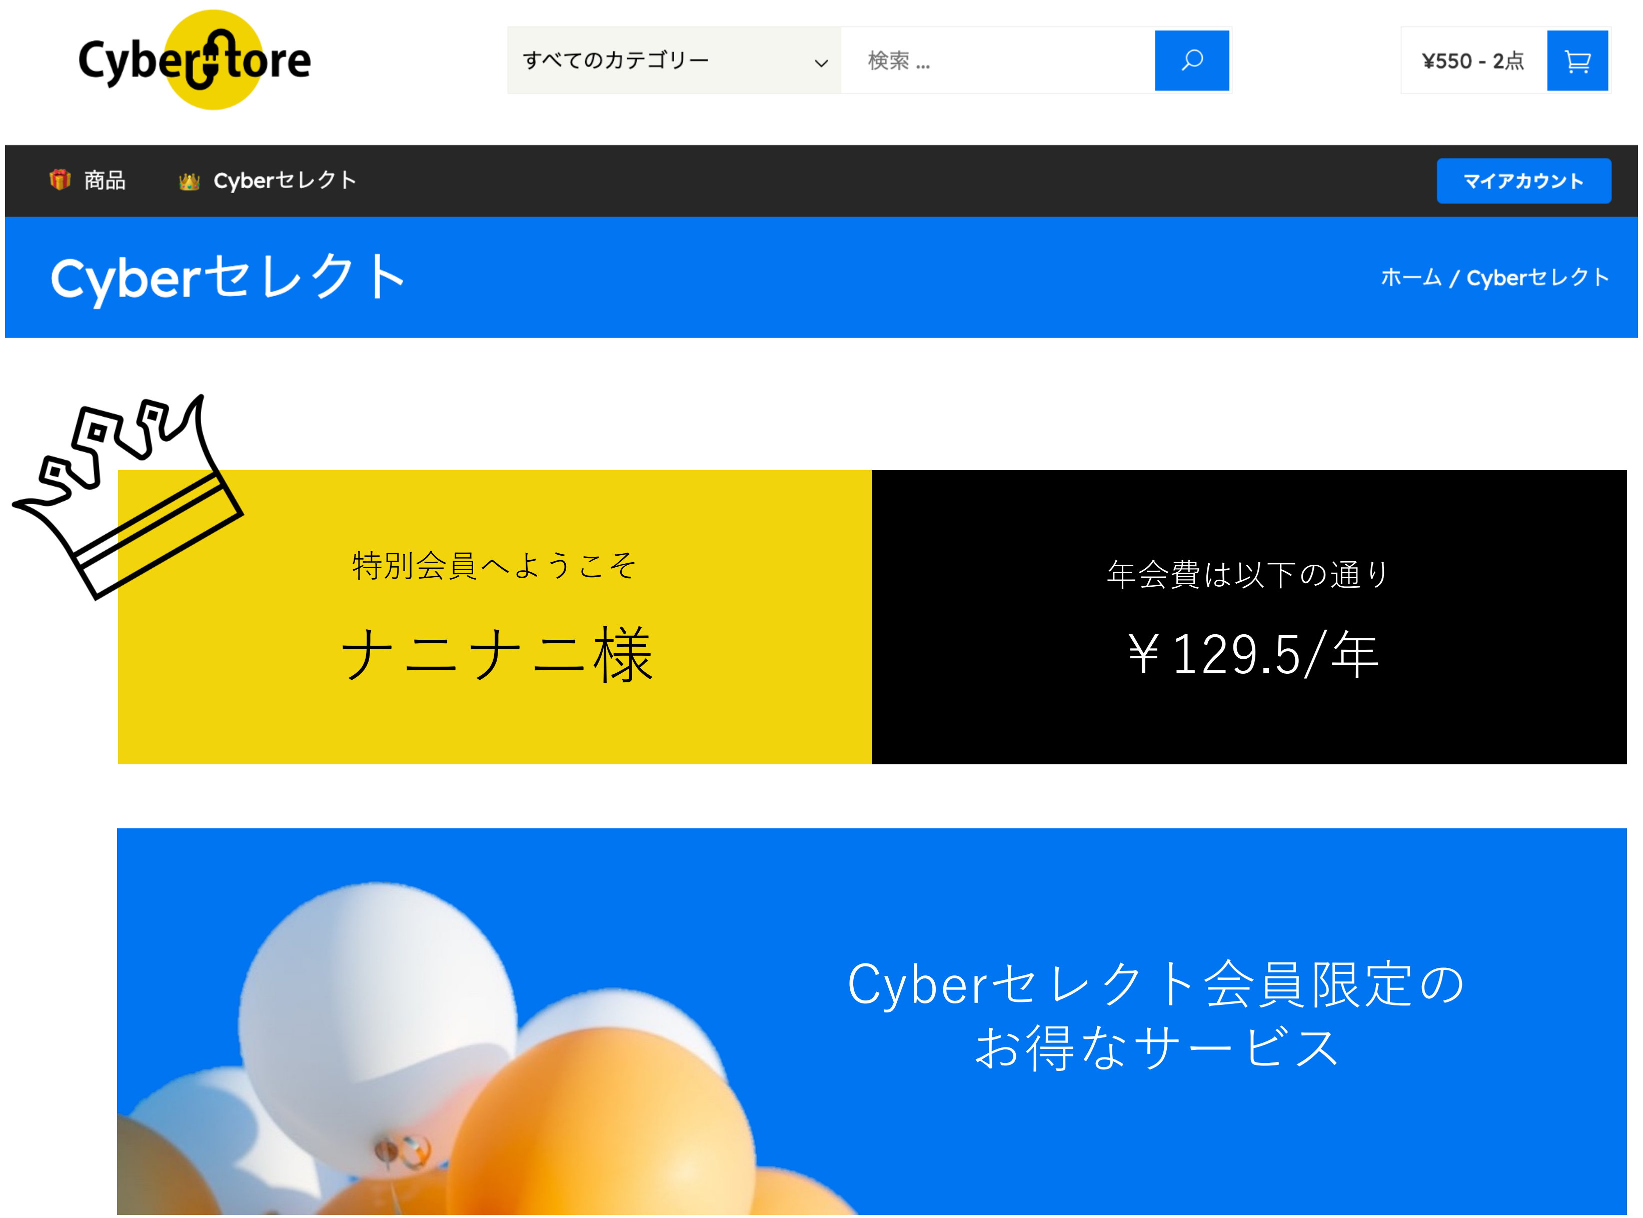

3

Check-out and sign up

チェックアウトとサインアップ

**Linguistic Dead-End**

Alphabet Soup

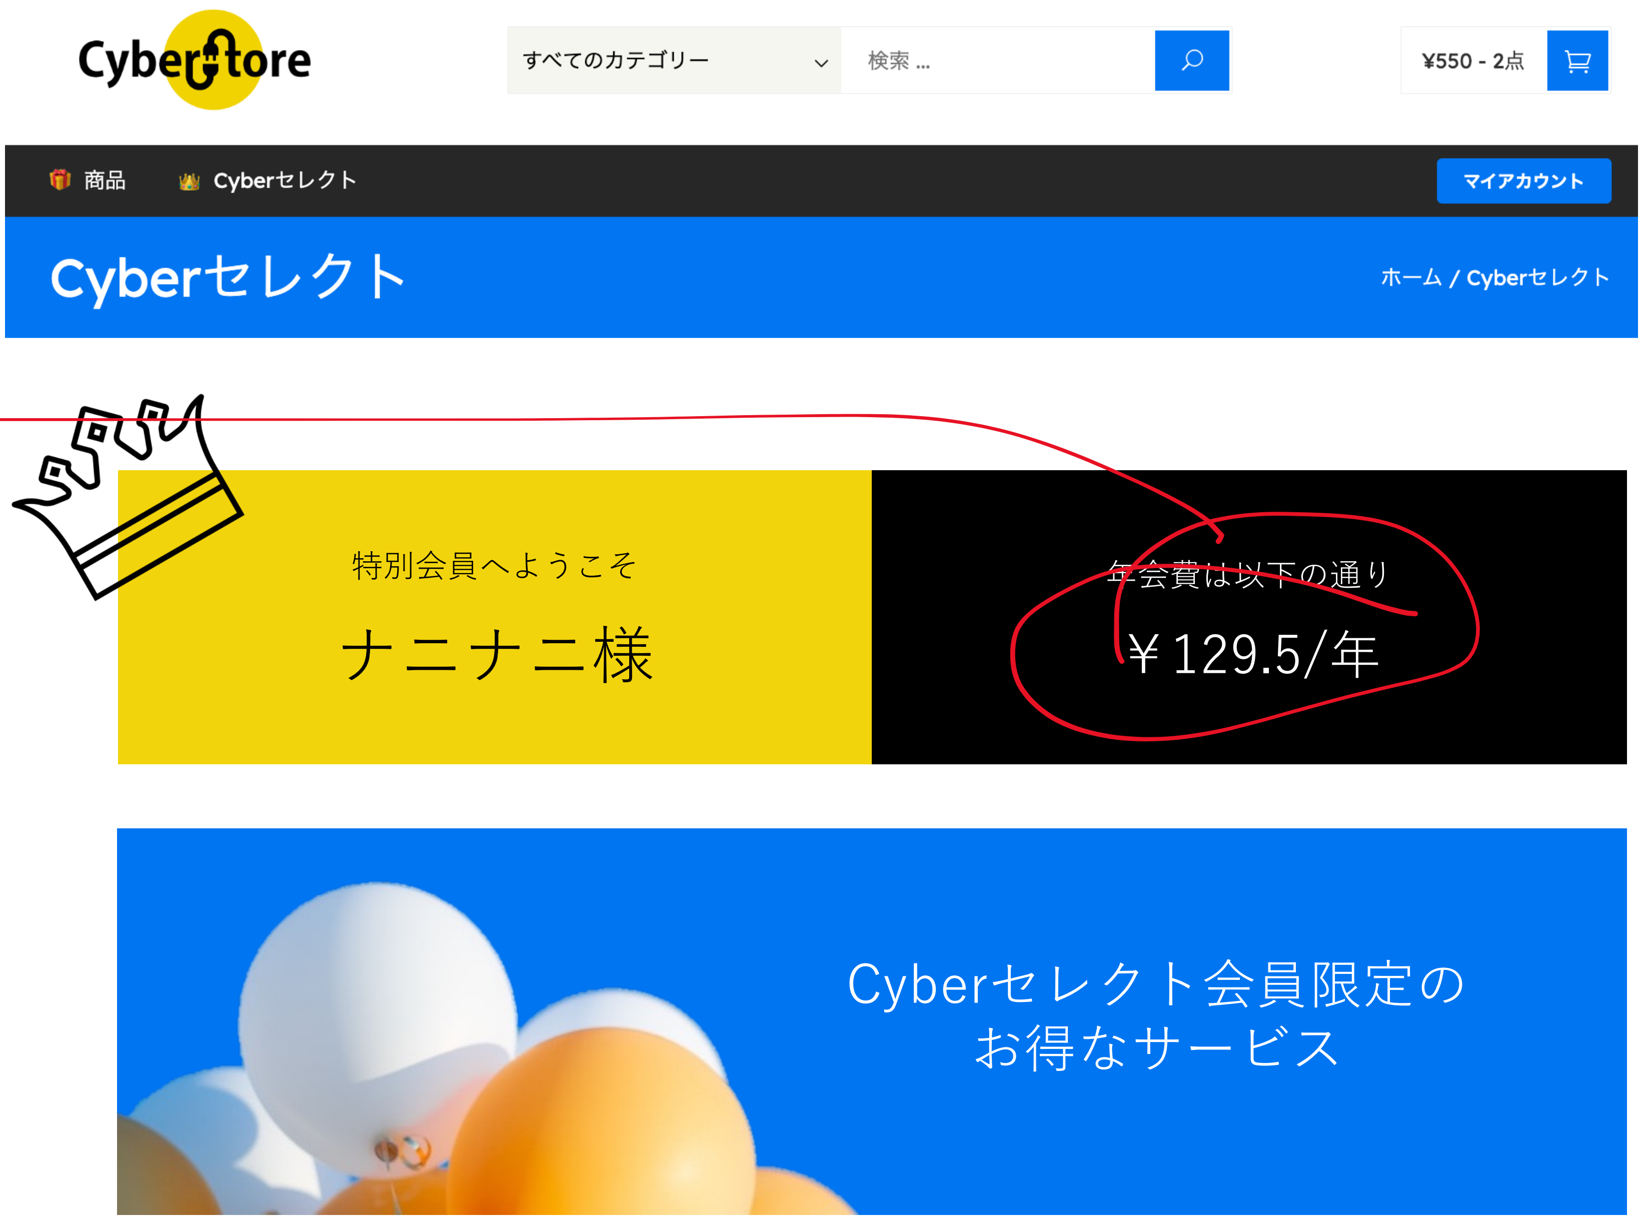

4

Cancel your membership

会員およびアカウントの解約

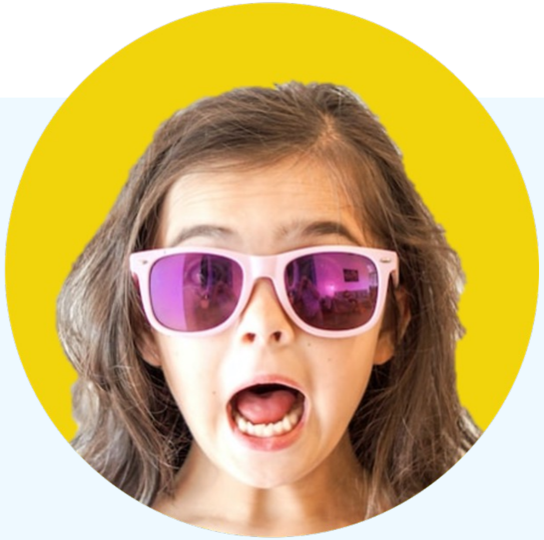

**なになに様、ご存じでしょうか？**

サイバーセレクトの会員期間はまだ**310日**残っています。

!

気をつけてください！解約すると、
サイバーセレクトに関する特別サービスが利用できなくなります。

4

Cancel your membership

会員およびアカウントの解約

**Interface Interference**

Confirmshaming

Toying with Emotions

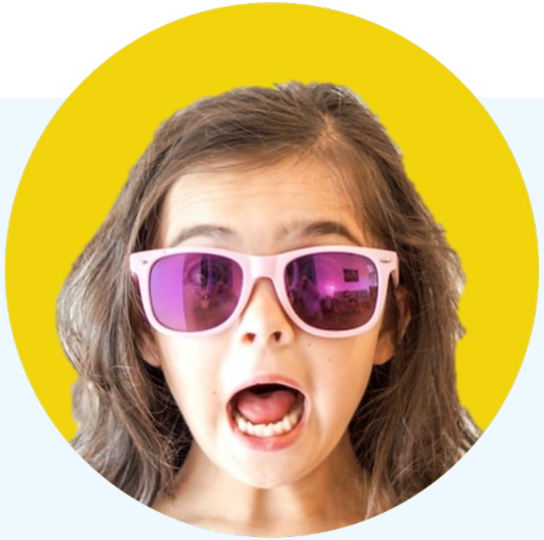

**なになに様、ご存じでしょうか？**

サイバーセレクトの会員期間はまだ**310日**残っています。

!

気をつけてください！解約すると、
サイバーセレクトに関する特別サービスが利用できなくなります。

4

Cancel your membership

会員およびアカウントの解約

これが、あなたが見逃すことになるものだ：

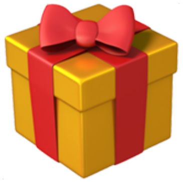

**特定のサービス**

お得なディールを
利用できなくなる

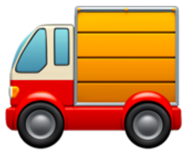

**送料無料**

送料はもうない！
送料がかかる

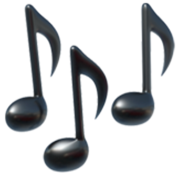

**OLUゴール**

数百万曲へのアクセスが
できなくなる。

**未体験のCyberセレクト特典はいますぐチェックしよう？**

**特典を維持する**

すべての利益を放棄する

4

Cancel your membership

会員およびアカウントの解約

**Interface Interference**

Confirmshaming

Toying with Emotions

False Hierarchy

これが、あなたが見逃すことになるものだ：

**特定のサービス**

お得なディールを
利用できなくなる

**送料無料**

送料はもうない！
送料がかかる

**OLUゴール**

数百万曲へのアクセスが
できなくなる。

**未体験のCyberセレクト特典はいますぐチェックしよう？**

**特典を維持する**

すべての利益を放棄する

4

Cancel your membership

会員およびアカウントの解約

お別れするのは残念です

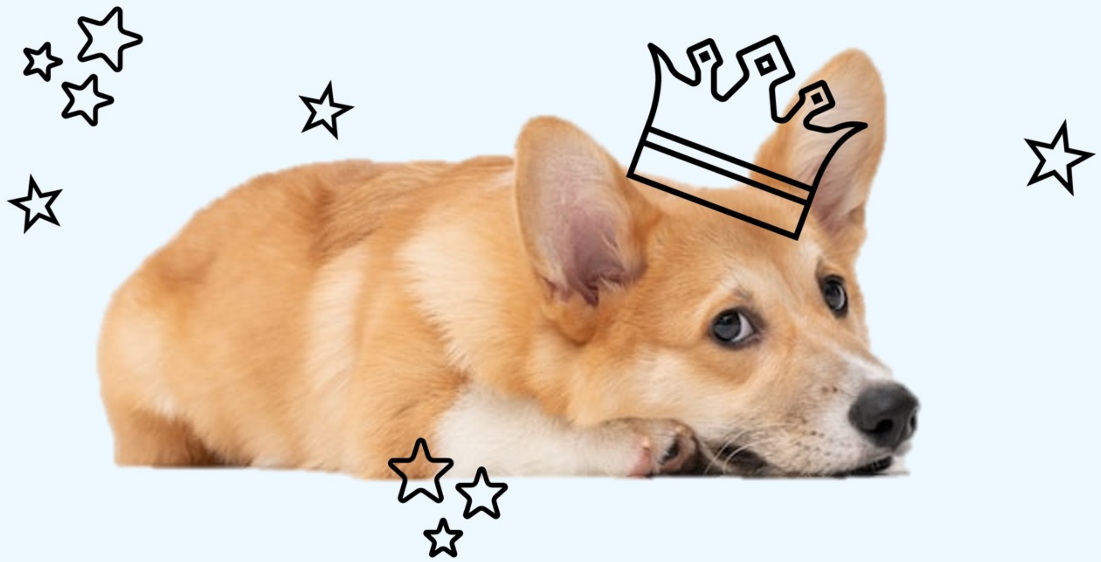

Cyberセレクトを再考する

HPに戻ろう

4

Cancel your membership

会員およびアカウントの解約

**Interface Interference**

Confirmshaming

Toying with Emotions

False Hierarchy

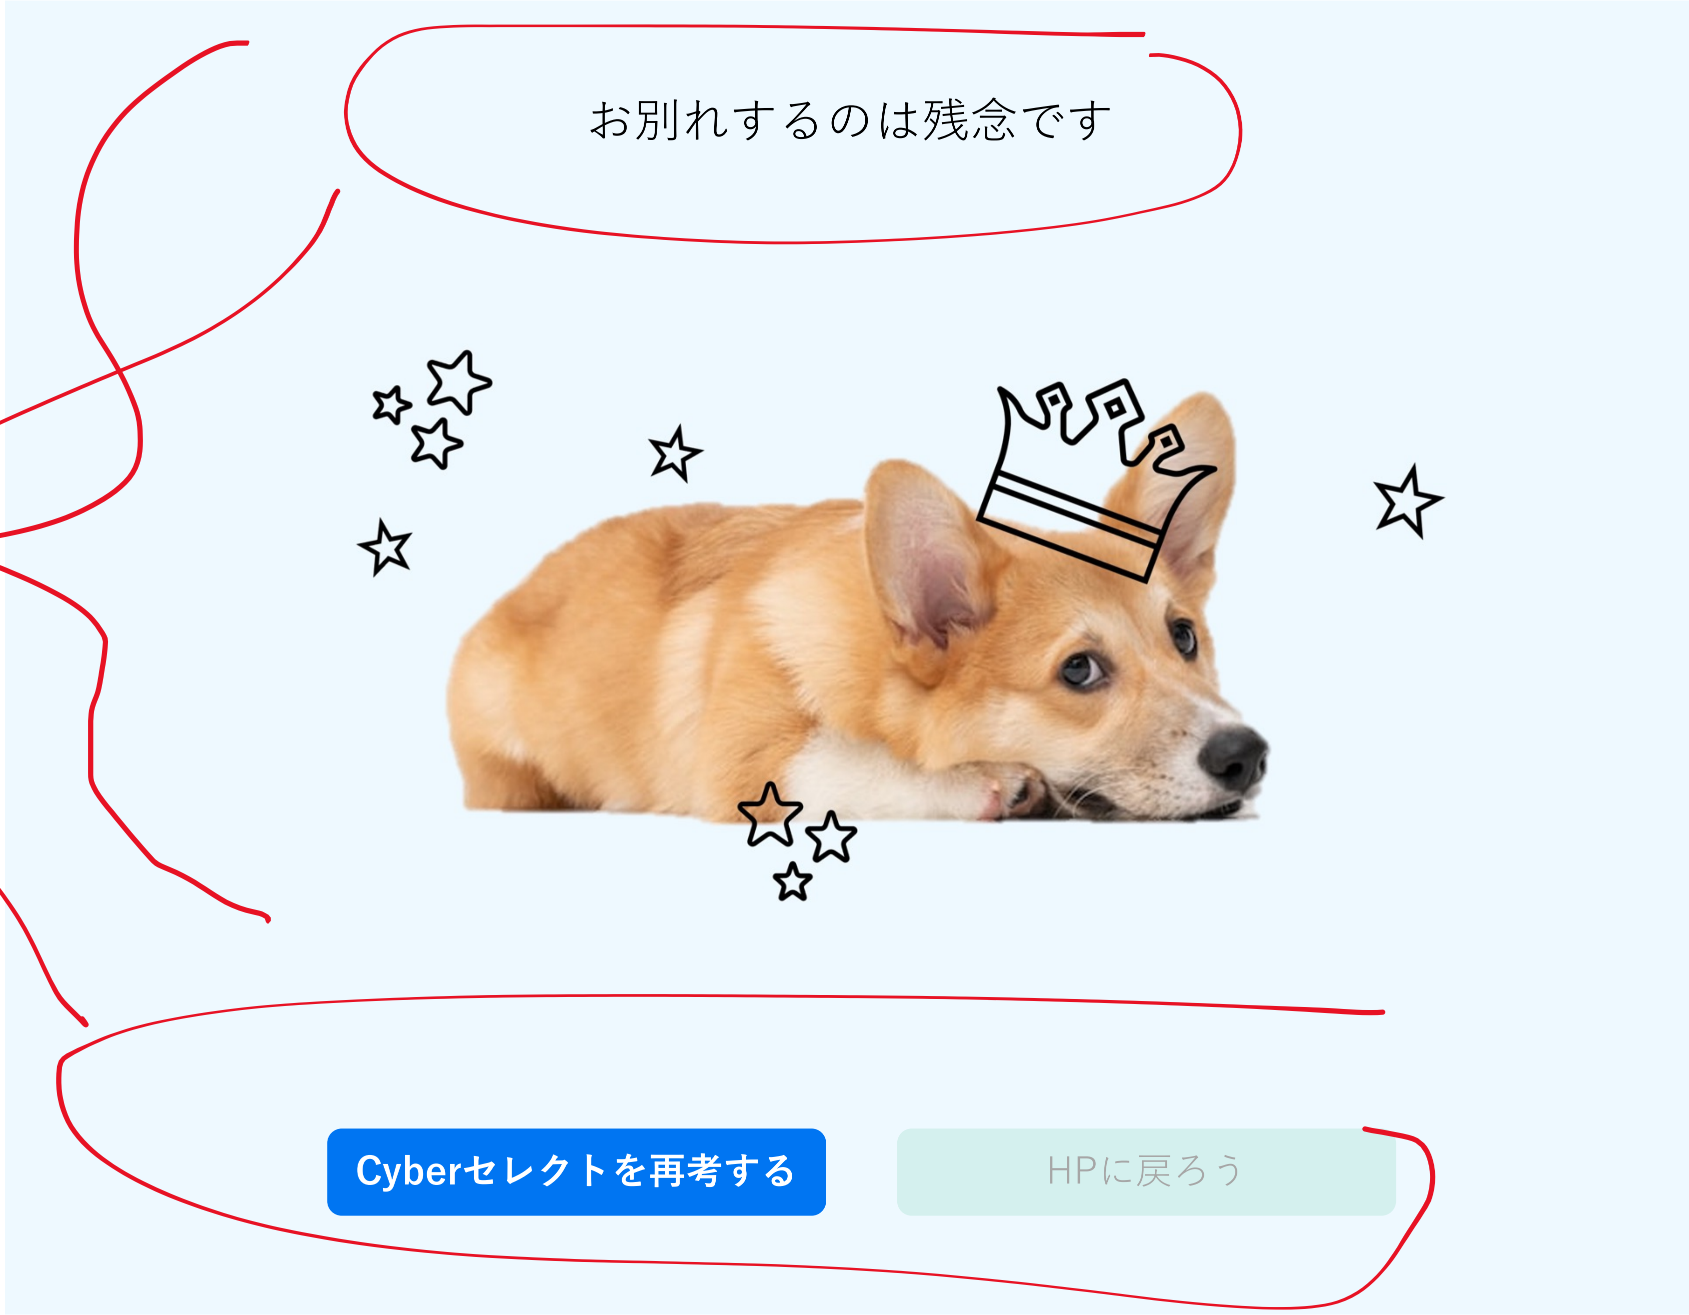

4

## Cancel your membership

会員およびアカウントの解約

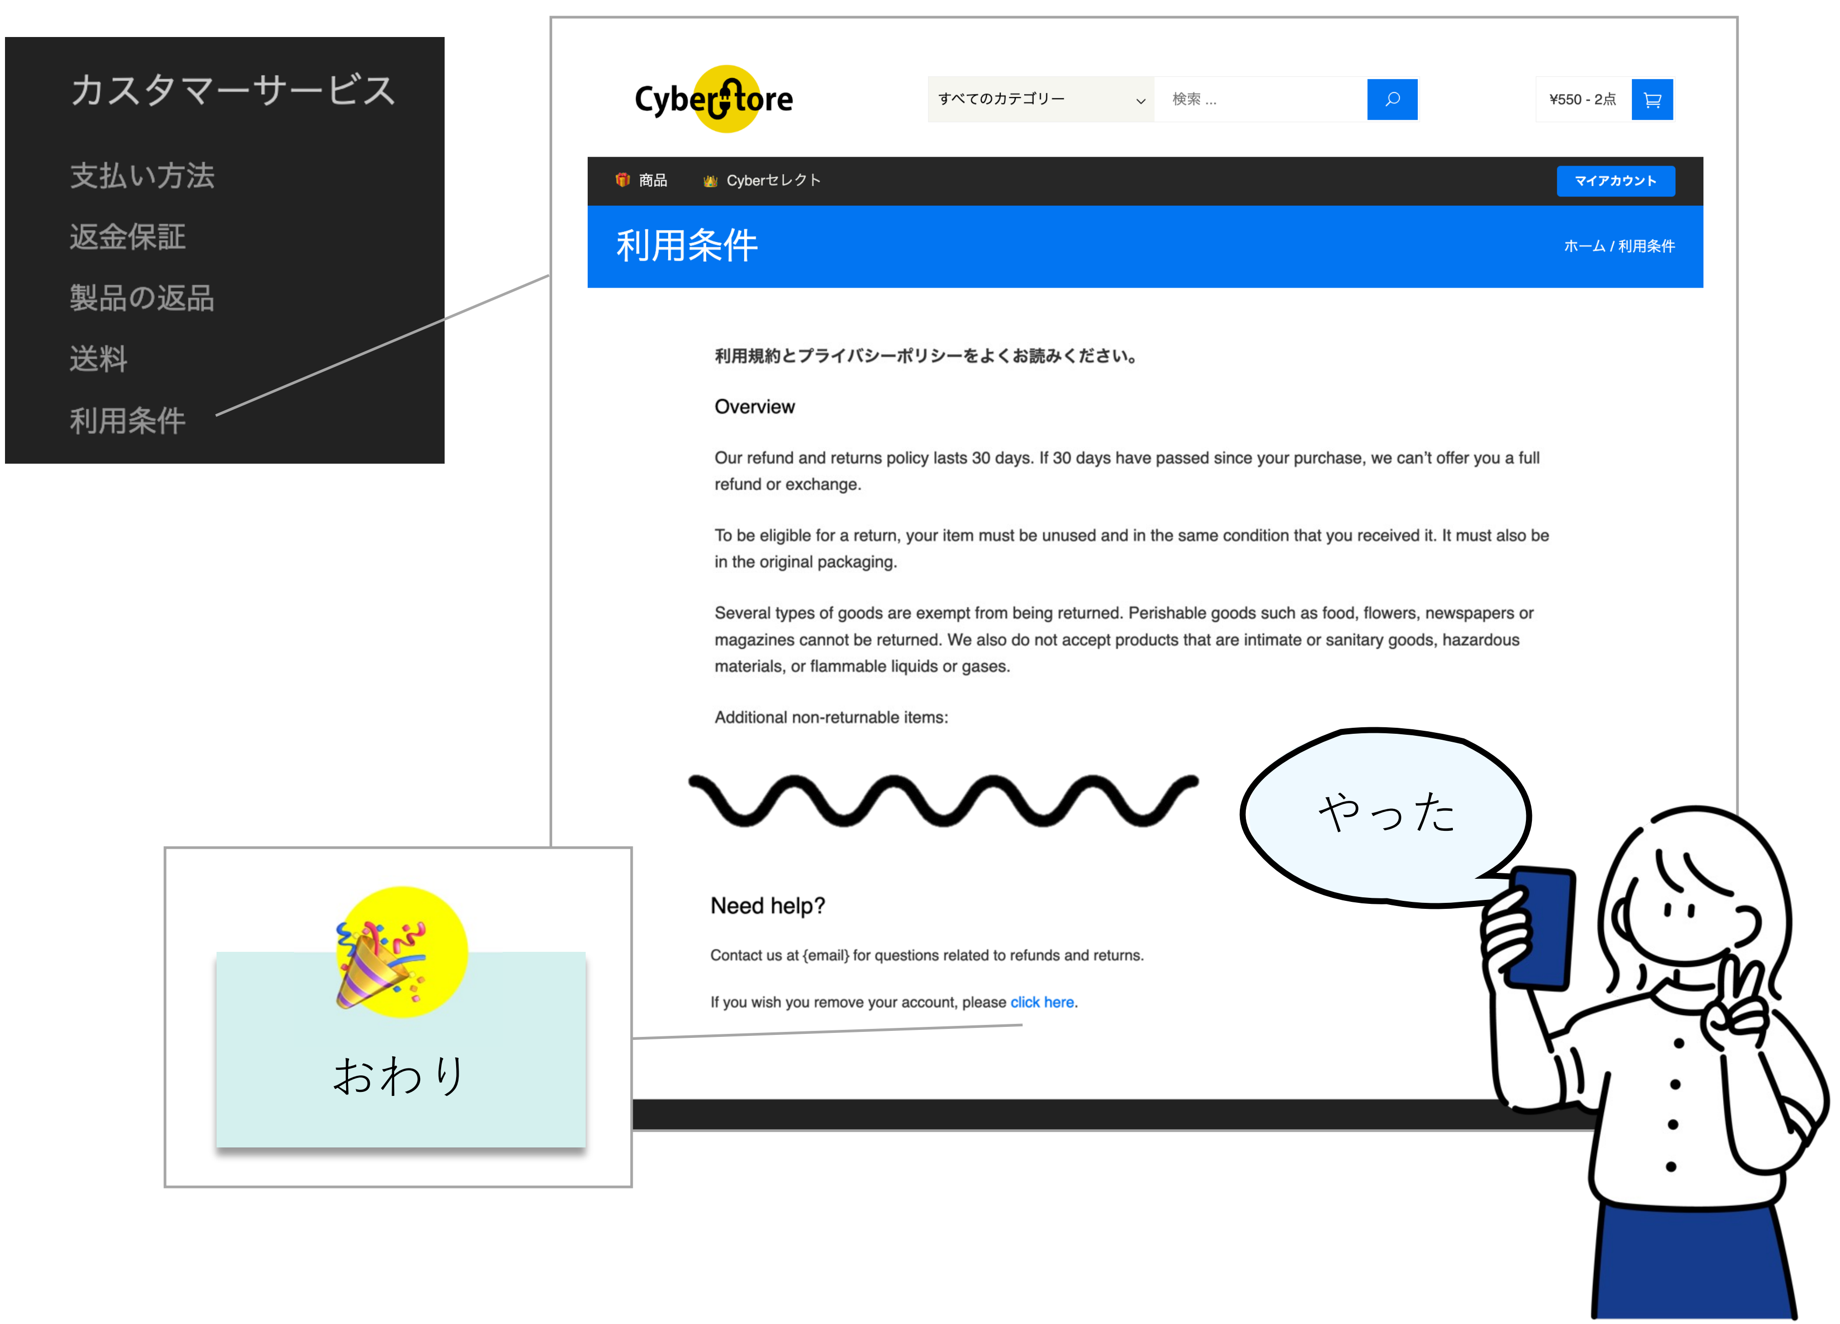

4

Cancel your membership

会員およびアカウントの解約

**Obstruction**
Hard to Cancel

**Linguistic Dead-Ends**
Untranslation

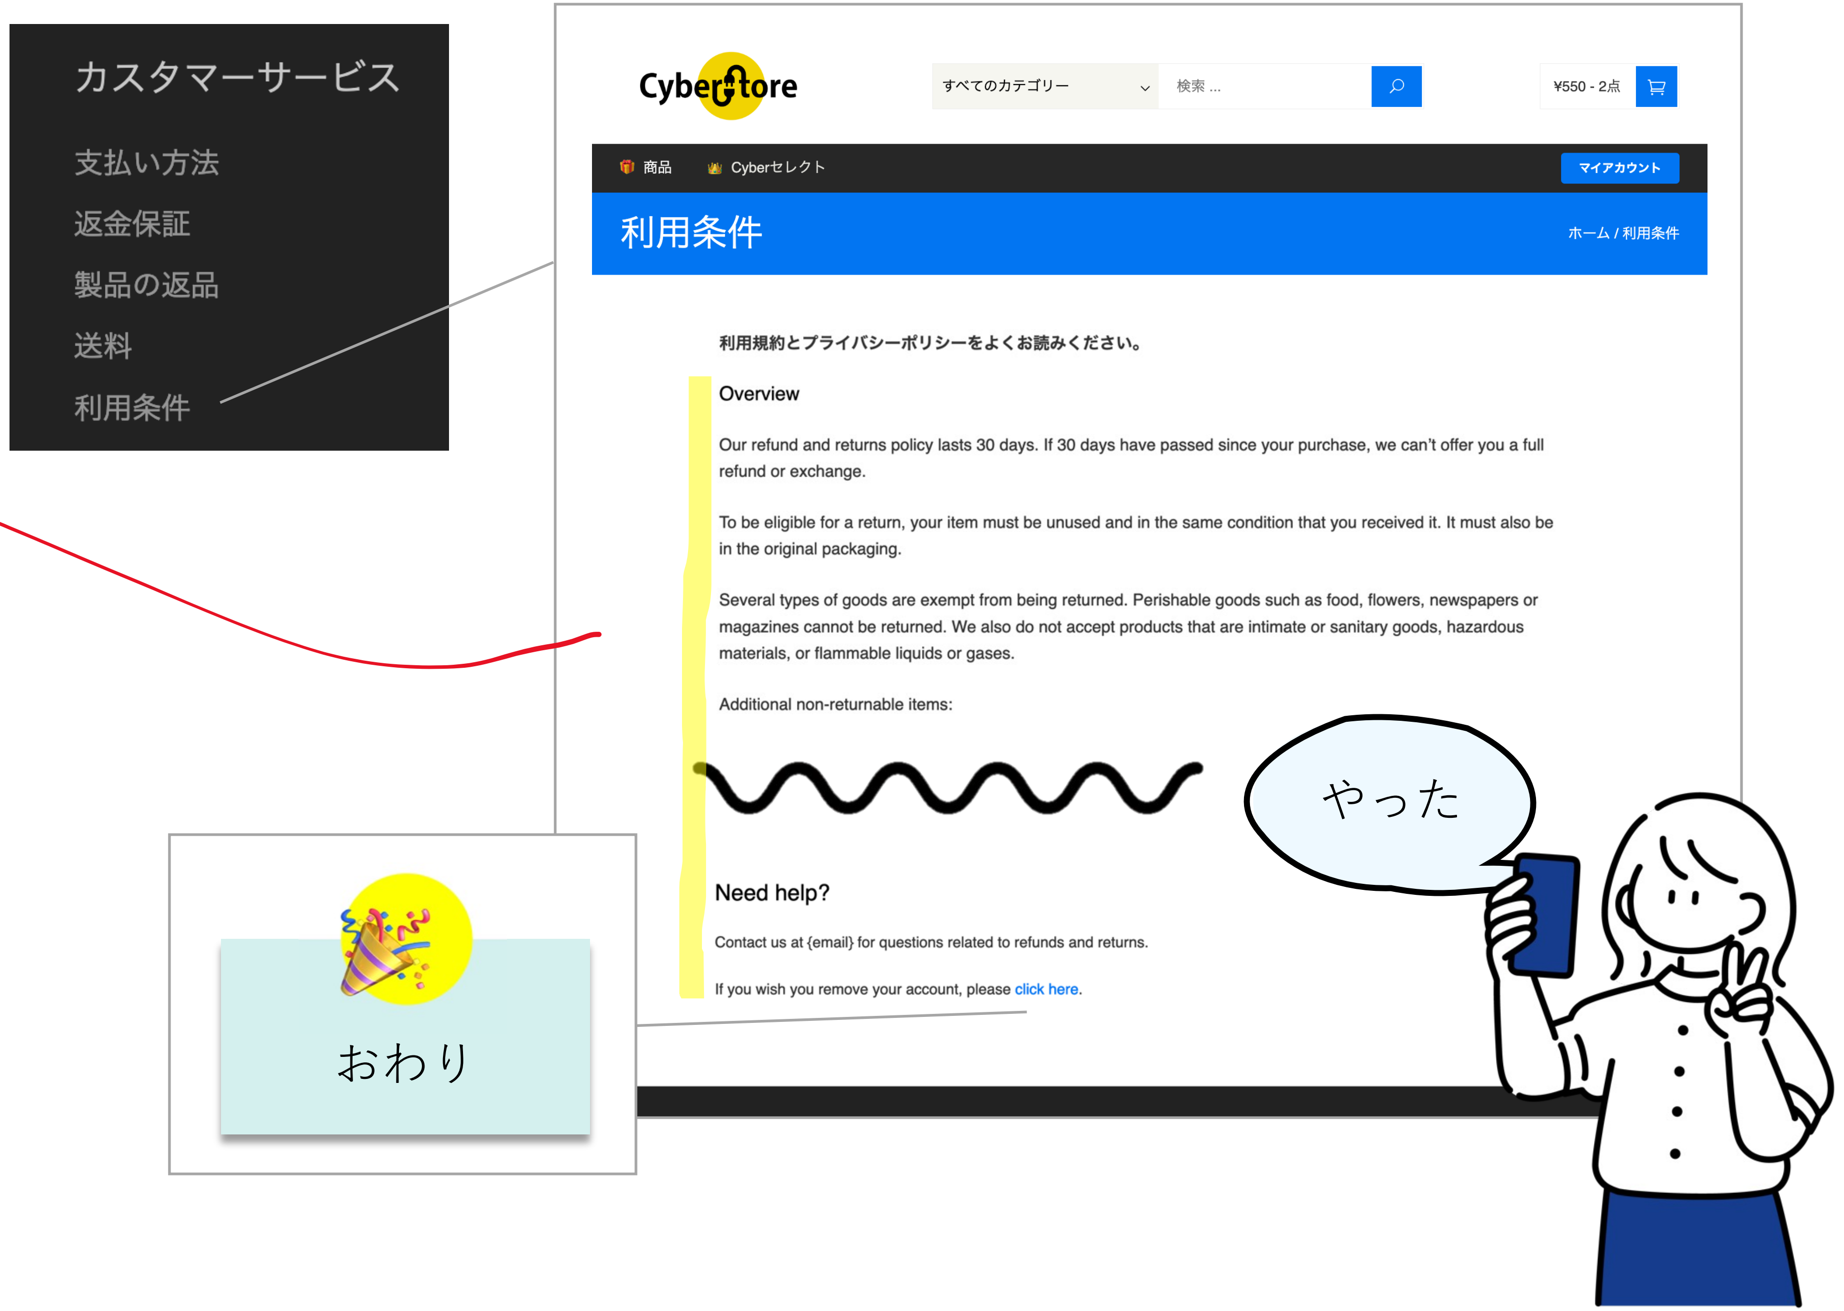

Supplement: Supplementary file 1 [file SM-DP_Cases.pdf]
